# Supplementary material for: Quantum tomography benchmarking
Source: arXiv:2012.15656 source file (2021-10-11)
Supplement: Supplementary file 1 [file Supplementary1.pdf]

# Supplementary material I. Methods analysis results

Quantum tomography benchmarking

Bantysh B. I., Chernyavskiy A. Yu., Bogdanov Yu. I.

The current document summarizes the results of using the quantum tomography (QT) benchmarking software for analyzing different QT methods. For each method we also provide a basic information: measurement protocol, quantum state estimator, data processing algorithm and computing machine. The sign "*" in tables means that the value was obtained by linear extrapolation of the dependence of $\log[1-F]_{95}$ on $\log N$.

## Contents

**1 MUB-FRML** **2**
1.1 1 qubit . . . 2
1.2 2 qubits . . . 3
1.3 3 qubits . . . 4

**2 FMUB-PPI** **5**
2.1 1 qubit . . . 5
2.2 2 qubits . . . 6
2.3 3 qubits . . . 7

**3 FMUB-FRLS** **7**
3.1 1 qubit . . . 8
3.2 2 qubits . . . 8
3.3 3 qubits . . . 9

**4 FMUB-FRML** **10**
4.1 1 qubit . . . 10
4.2 2 qubits . . . 11
4.3 3 qubits . . . 12

**5 FMUB-TRML** **12**
5.1 1 qubit . . . 13
5.2 2 qubits . . . 14
5.3 3 qubits . . . 14

**6 FMUB-ARML** **15**
6.1 1 qubit . . . 15
6.2 2 qubits . . . 16
6.3 3 qubits . . . 17

**7 FMUB-CS** **18**
7.1 1 qubit . . . 18
7.2 2 qubits . . . 19
7.3 3 qubits . . . 20

**8 Pauli-CS** **20**
8.1 1 qubit . . . 21
8.2 2 qubits . . . 21
8.3 3 qubits . . . 22

**9 AMUB-FRML** **23**
9.1 1 qubit . . . 23
9.2 2 qubits . . . 24
9.3 3 qubits . . . 25

**10 FO-FRML** **25**
10.1 2 qubits . . . 26
10.2 3 qubits . . . 27

**11 FOMUB-FRML** **27**
11.1 2 qubits . . . 28
11.2 3 qubits . . . 28

**12 SGQT** **29**
12.1 1 qubit . . . 29
12.2 2 qubits . . . 30
12.3 3 qubits . . . 30

# 1 MUB-FRML

- Protocol: mutually unbiased bases
- Estimator: full-rank maximum likelihood
- Algorithm: full-rank root approach estimator using [8]
- Machine: Intel(R) Core(TM) i5-7200U CPU @ 2.50GHz

## 1.1 1 qubit

Table 1: MUB-FRML, 1 qubit, random pure states

| $F_B, \%$ | $N_B$ | $M_B$ | $T_{P,B}$, sec | $T_{E,B}$, sec | $\eta_B$ | $O_B$ |
|---|---|---|---|---|---|---|
| 90 | *83 | – | – | – | – | – |
| 99 | 9 881 | 3 | 0.00053 | 0.0055 | 0.045 | 0 |
| 99.9 | 867 389 | 3 | 0.00049 | 0.0052 | 0.005 | 0 |
| 99.99 | *2 589 235 | – | – | – | – | – |

Table 2: MUB-FRML, 1 qubit, random mixed states by partial tracing (rank-2) test

| $F_B, \%$ | $N_B$ | $M_B$ | $T_{P,B}$, sec | $T_{E,B}$, sec | $\eta_B$ | $O_B$ |
|---|---|---|---|---|---|---|
| 90 | *48 | – | – | – | – | – |
| 99 | 1 109 | 3 | 0.00028 | 0.0031 | 0.65 | 0.03 |
| 99.9 | 10 126 | 3 | 0.00031 | 0.0033 | 0.62 | 0.037 |
| 99.99 | 106 277 | 3 | 0.00028 | 0.0031 | 0.5 | 0.037 |

Table 3: MUB-FRML, 1 qubit, random mixed states by partial tracing (full-rank) test

| $F_B, \%$ | $N_B$ | $M_B$ | $T_{P,B}$, sec | $T_{E,B}$, sec | $\eta_B$ | $O_B$ |
|---|---|---|---|---|---|---|
| 90 | *62 | – | – | – | – | – |
| 99 | 994 | 3 | 0.00028 | 0.0031 | 0.67 | 0.028 |
| 99.9 | 11 637 | 3 | 0.00029 | 0.0032 | 0.58 | 0.033 |
| 99.99 | 134 940 | 3 | 0.00029 | 0.0033 | 0.42 | 0.046 |

Table 4: MUB-FRML, 1 qubit, random noisy preparation

| $F_B, \%$ | $N_B$ | $M_B$ | $T_{P,B}$, sec | $T_{E,B}$, sec | $\eta_B$ | $O_B$ |
|---|---|---|---|---|---|---|
| 90 | *19 | – | – | – | – | – |
| 99 | 2 252 | 3 | 0.00026 | 0.0032 | 0.38 | 0.017 |
| 99.9 | 27 014 | 3 | 0.00027 | 0.0031 | 0.3 | 0.037 |
| 99.99 | 264 308 | 3 | 0.00026 | 0.003 | 0.28 | 0.03 |

### 1.2 2 qubits

Table 5: MUB-FRML, 2 qubits, random pure states

| $F_B, \%$ | $N_B$ | $M_B$ | $T_{P,B}$, sec | $T_{E,B}$, sec | $\eta_B$ | $O_B$ |
|---|---|---|---|---|---|---|
| 90 | 381 | 5 | 0.00057 | 0.029 | 0.18 | 0.0017 |
| 99 | 33 864 | 5 | 0.00061 | 0.16 | 0.02 | 0.0029 |
| 99.9 | *1 638 550 | – | – | – | – | – |
| 99.99 | *2 748 077 | – | – | – | – | – |

Table 6: MUB-FRML, 2 qubits, random mixed states by partial tracing (rank-2) test

| $F_B, \%$ | $N_B$ | $M_B$ | $T_{P,B}$, sec | $T_{E,B}$, sec | $\eta_B$ | $O_B$ |
|---|---|---|---|---|---|---|
| 90 | 468 | 5 | 0.00061 | 0.023 | 0.45 | 0.005 |
| 99 | 36 589 | 5 | 0.0006 | 0.094 | 0.066 | 0.0023 |
| 99.9 | *1 619 547 | – | – | – | – | – |
| 99.99 | *2 708 766 | – | – | – | – | – |

Table 7: MUB-FRML, 2 qubits, random mixed states by partial tracing (full-rank) test

| $F_B$, % | $N_B$ | $M_B$ | $T_{P,B}$, sec | $T_{E,B}$, sec | $\eta_B$ | $O_B$ |
|---|---|---|---|---|---|---|
| 90 | *143 | – | – | – | – | – |
| 99 | 10 061 | 5 | 0.00077 | 0.0081 | 0.45 | 0.02 |
| 99.9 | 160 266 | 5 | 0.00073 | 0.0064 | 0.35 | 0.061 |
| 99.99 | 2 066 031 | 5 | 0.00077 | 0.0057 | 0.28 | 0.071 |

Table 8: MUB-FRML, 2 qubits, random noisy preparation

| $F_B$, % | $N_B$ | $M_B$ | $T_{P,B}$, sec | $T_{E,B}$, sec | $\eta_B$ | $O_B$ |
|---|---|---|---|---|---|---|
| 90 | *173 | – | – | – | – | – |
| 99 | 25 148 | 5 | 0.00066 | 0.036 | 0.16 | 0.014 |
| 99.9 | 1 016 042 | 5 | 0.00067 | 0.022 | 0.072 | 0.056 |
| 99.99 | 9 327 501 | 5 | 0.00061 | 0.0053 | 0.07 | 0.063 |

### 1.3 3 qubits

Table 9: MUB-FRML, 3 qubits, random pure states

| $F_B$, % | $N_B$ | $M_B$ | $T_{P,B}$, sec | $T_{E,B}$, sec | $\eta_B$ | $O_B$ |
|---|---|---|---|---|---|---|
| 90 | 903 | 9 | 0.00054 | 0.076 | 0.13 | 0.0022 |
| 99 | 83 906 | 9 | 0.00055 | 0.55 | 0.014 | 0.0038 |
| 99.9 | *2 007 764 | – | – | – | – | – |
| 99.99 | *2 793 700 | – | – | – | – | – |

Table 10: MUB-FRML, 3 qubits, random mixed states by partial tracing (rank-2) test

| $F_B$, % | $N_B$ | $M_B$ | $T_{P,B}$, sec | $T_{E,B}$, sec | $\eta_B$ | $O_B$ |
|---|---|---|---|---|---|---|
| 90 | 1 836 | 9 | 0.00057 | 0.13 | 0.22 | 0.0061 |
| 99 | 164 625 | 9 | 0.00053 | 0.68 | 0.025 | 0.008 |
| 99.9 | *12 623 083 | – | – | – | – | – |
| 99.99 | *26 681 907 | – | – | – | – | – |

Table 11: MUB-FRML, 3 qubits, random mixed states by partial tracing (full-rank) test

| $F_B$, % | $N_B$ | $M_B$ | $T_{P,B}$, sec | $T_{E,B}$, sec | $\eta_B$ | $O_B$ |
|---|---|---|---|---|---|---|
| 90 | *112 | – | – | – | – | – |
| 99 | 58 098 | 9 | 0.00065 | 0.08 | 0.4 | 0.0044 |
| 99.9 | 1 197 954 | 9 | 0.0007 | 0.041 | 0.28 | 0.05 |
| 99.99 | 19 227 538 | 9 | 0.00066 | 0.015 | 0.22 | 0.074 |

Table 12: MUB-FRML, 3 qubits, random noisy preparation

| $F_B, \%$ | $N_B$ | $M_B$ | $T_{P,B}$, sec | $T_{E,B}$, sec | $\eta_B$ | $O_B$ |
|---|---|---|---|---|---|---|
| 90 | *177 | – | – | – | – | – |
| 99 | 167 081 | 9 | 0.0012 | 0.8 | 0.12 | 0.016 |
| 99.9 | 12 349 241 | 9 | 0.0012 | 0.75 | 0.027 | 0.0047 |
| 99.99 | *126 680 555 | – | – | – | – | – |

# 2 FMUB-PPI

- Protocol: factorized mutually unbiased bases
- Estimator: projected pseudo-inversion
- Algorithm: linear inversion with projection to simplex using subroutine from [6]
- Machine: Intel(R) Core(TM) i5-7200U CPU @ 2.50GHz

## 2.1 1 qubit

Table 13: FMUB-PPI, 1 qubit, random pure states

| $F_B, \%$ | $N_B$ | $M_B$ | $T_{P,B}$, sec | $T_{E,B}$, sec | $\eta_B$ | $O_B$ |
|---|---|---|---|---|---|---|
| 90 | *83 | – | – | – | – | – |
| 99 | 9 881 | 3 | 0.00035 | 0.0006 | 0.045 | 0 |
| 99.9 | 867 383 | 3 | 0.00035 | 0.00055 | 0.005 | 0 |
| 99.99 | *2 589 225 | – | – | – | – | – |

Table 14: FMUB-PPI, 1 qubit, random mixed states by partial tracing (rank-2) test

| $F_B, \%$ | $N_B$ | $M_B$ | $T_{P,B}$, sec | $T_{E,B}$, sec | $\eta_B$ | $O_B$ |
|---|---|---|---|---|---|---|
| 90 | *47 | – | – | – | – | – |
| 99 | 1 110 | 3 | 0.00032 | 0.00053 | 0.65 | 0.03 |
| 99.9 | 10 126 | 3 | 0.00033 | 0.00059 | 0.62 | 0.036 |
| 99.99 | 106 277 | 3 | 0.00034 | 0.00053 | 0.5 | 0.037 |

Table 15: FMUB-PPI, 1 qubit, random mixed states by partial tracing (full-rank) test

| $F_B, \%$ | $N_B$ | $M_B$ | $T_{P,B}$, sec | $T_{E,B}$, sec | $\eta_B$ | $O_B$ |
|---|---|---|---|---|---|---|
| 90 | *65 | – | – | – | – | – |
| 99 | 1 015 | 3 | 0.00031 | 0.00051 | 0.67 | 0.027 |
| 99.9 | 11 714 | 3 | 0.00032 | 0.00057 | 0.58 | 0.033 |
| 99.99 | 134 940 | 3 | 0.00031 | 0.00048 | 0.42 | 0.046 |

Table 16: FMUB-PPI, 1 qubit, random noisy preparation

| $F_B, \%$ | $N_B$ | $M_B$ | $T_{P,B}$, sec | $T_{E,B}$, sec | $\eta_B$ | $O_B$ |
|---|---|---|---|---|---|---|
| 90 | *19 | – | – | – | – | – |
| 99 | 2 262 | 3 | 0.00041 | 0.00078 | 0.37 | 0.017 |
| 99.9 | 27 014 | 3 | 0.00043 | 0.0008 | 0.3 | 0.037 |
| 99.99 | 264 308 | 3 | 0.00043 | 0.00079 | 0.28 | 0.03 |

### 2.2 2 qubits

Table 17: FMUB-PPI, 2 qubits, random pure states

| $F_B, \%$ | $N_B$ | $M_B$ | $T_{P,B}$, sec | $T_{E,B}$, sec | $\eta_B$ | $O_B$ |
|---|---|---|---|---|---|---|
| 90 | 568 | 9 | 0.00064 | 0.00055 | 0.12 | 0.0015 |
| 99 | 50 976 | 9 | 0.00063 | 0.00056 | 0.013 | 0.0027 |
| 99.9 | *1 811 355 | – | – | – | – | – |
| 99.99 | *2 770 068 | – | – | – | – | – |

Table 18: FMUB-PPI, 2 qubits, random mixed states by partial tracing (rank-2) test

| $F_B, \%$ | $N_B$ | $M_B$ | $T_{P,B}$, sec | $T_{E,B}$, sec | $\eta_B$ | $O_B$ |
|---|---|---|---|---|---|---|
| 90 | 642 | 9 | 0.00062 | 0.00056 | 0.33 | 0.0026 |
| 99 | 51 126 | 9 | 0.00063 | 0.00054 | 0.048 | 0.00058 |
| 99.9 | *1 782 349 | – | – | – | – | – |
| 99.99 | *2 727 413 | – | – | – | – | – |

Table 19: FMUB-PPI, 2 qubits, random mixed states by partial tracing (full-rank) test

| $F_B, \%$ | $N_B$ | $M_B$ | $T_{P,B}$, sec | $T_{E,B}$, sec | $\eta_B$ | $O_B$ |
|---|---|---|---|---|---|---|
| 90 | *346 | – | – | – | – | – |
| 99 | 16 172 | 9 | 0.0006 | 0.00053 | 0.31 | 0.029 |
| 99.9 | 265 894 | 9 | 0.00061 | 0.00055 | 0.23 | 0.057 |
| 99.99 | 3 554 953 | 9 | 0.00061 | 0.00052 | 0.18 | 0.074 |

Table 20: FMUB-PPI, 2 qubits, random noisy preparation

| $F_B, \%$ | $N_B$ | $M_B$ | $T_{P,B}$, sec | $T_{E,B}$, sec | $\eta_B$ | $O_B$ |
|---|---|---|---|---|---|---|
| 90 | *189 | – | – | – | – | – |
| 99 | 37 925 | 9 | 0.00062 | 0.00053 | 0.1 | 0.011 |
| 99.9 | 1 400 187 | 9 | 0.00061 | 0.00057 | 0.049 | 0.038 |
| 99.99 | *10 765 217 | – | – | – | – | – |

### 2.3 3 qubits

Table 21: FMUB-PPI, 3 qubits, random pure states

| $F_B$, % | $N_B$ | $M_B$ | $T_{P,B}$, sec | $T_{E,B}$, sec | $\eta_B$ | $O_B$ |
|---:|---:|---:|---:|---:|---:|---:|
| 90 | 2 134 | 27 | 0.0025 | 0.0034 | 0.053 | 0.0077 |
| 99 | 203 021 | 27 | 0.0025 | 0.0036 | 0.0056 | 0.019 |
| 99.9 | *2 300 913 | – | – | – | – | – |
| 99.99 | *2 847 883 | – | – | – | – | – |

Table 22: FMUB-PPI, 3 qubits, random mixed states by partial tracing (rank-2) test

| $F_B$, % | $N_B$ | $M_B$ | $T_{P,B}$, sec | $T_{E,B}$, sec | $\eta_B$ | $O_B$ |
|---:|---:|---:|---:|---:|---:|---:|
| 90 | 3 708 | 27 | 0.0018 | 0.0026 | 0.11 | 0.0071 |
| 99 | 337 607 | 27 | 0.0018 | 0.0026 | 0.012 | 0.0055 |
| 99.9 | *16 148 565 | – | – | – | – | – |
| 99.99 | *27 176 645 | – | – | – | – | – |

Table 23: FMUB-PPI, 3 qubits, random mixed states by partial tracing (full-rank) test

| $F_B$, % | $N_B$ | $M_B$ | $T_{P,B}$, sec | $T_{E,B}$, sec | $\eta_B$ | $O_B$ |
|---:|---:|---:|---:|---:|---:|---:|
| 90 | *1 598 | – | – | – | – | – |
| 99 | 111 638 | 27 | 0.0017 | 0.0027 | 0.22 | 0.0086 |
| 99.9 | 2 419 468 | 27 | 0.0016 | 0.0028 | 0.15 | 0.047 |
| 99.99 | 41 797 578 | 27 | 0.0017 | 0.0028 | 0.11 | 0.068 |

Table 24: FMUB-PPI, 3 qubits, random noisy preparation

| $F_B$, % | $N_B$ | $M_B$ | $T_{P,B}$, sec | $T_{E,B}$, sec | $\eta_B$ | $O_B$ |
|---:|---:|---:|---:|---:|---:|---:|
| 90 | *1 556 | – | – | – | – | – |
| 99 | 376 265 | 27 | 0.0017 | 0.0025 | 0.056 | 0.018 |
| 99.9 | 23 467 175 | 27 | 0.0016 | 0.0025 | 0.014 | 0.0093 |
| 99.99 | *148 667 382 | – | – | – | – | – |

# 3 FMUB-FRLS

- Protocol: factorized mutually unbiased bases
- Estimator: full-rank least squares
- Algorithm: least squares convex optimization using [7]
- Machine: Intel(R) Core(TM) i5-7200U CPU @ 2.50GHz

### 3.1 1 qubit

Table 25: FMUB-FRLS, 1 qubit, random pure states

| $F_B, \%$ | $N_B$ | $M_B$ | $T_{P,B}$, sec | $T_{E,B}$, sec | $\eta_B$ | $O_B$ |
|---|---|---|---|---|---|---|
| 90 | *83 | – | – | – | – | – |
| 99 | 9 881 | 3 | 0.00045 | 0.54 | 0.045 | 0 |
| 99.9 | 867 380 | 3 | 0.00042 | 0.55 | 0.005 | 0 |
| 99.99 | *2 589 217 | – | – | – | – | – |

Table 26: FMUB-FRLS, 1 qubit, random mixed states by partial tracing (rank-2) test

| $F_B, \%$ | $N_B$ | $M_B$ | $T_{P,B}$, sec | $T_{E,B}$, sec | $\eta_B$ | $O_B$ |
|---|---|---|---|---|---|---|
| 90 | *47 | – | – | – | – | – |
| 99 | 1 110 | 3 | 0.00045 | 0.53 | 0.65 | 0.03 |
| 99.9 | 10 126 | 3 | 0.00041 | 0.53 | 0.62 | 0.036 |
| 99.99 | 106 277 | 3 | 0.00043 | 0.54 | 0.5 | 0.037 |

Table 27: FMUB-FRLS, 1 qubit, random mixed states by partial tracing (full-rank) test

| $F_B, \%$ | $N_B$ | $M_B$ | $T_{P,B}$, sec | $T_{E,B}$, sec | $\eta_B$ | $O_B$ |
|---|---|---|---|---|---|---|
| 90 | *65 | – | – | – | – | – |
| 99 | 1 015 | 3 | 0.00034 | 0.41 | 0.66 | 0.027 |
| 99.9 | 11 704 | 3 | 0.00034 | 0.41 | 0.58 | 0.033 |
| 99.99 | 134 940 | 3 | 0.00033 | 0.42 | 0.42 | 0.046 |

Table 28: FMUB-FRLS, 1 qubit, random noisy preparation

| $F_B, \%$ | $N_B$ | $M_B$ | $T_{P,B}$, sec | $T_{E,B}$, sec | $\eta_B$ | $O_B$ |
|---|---|---|---|---|---|---|
| 90 | *19 | – | – | – | – | – |
| 99 | 2 261 | 3 | 0.00031 | 0.37 | 0.37 | 0.017 |
| 99.9 | 27 014 | 3 | 0.00032 | 0.37 | 0.3 | 0.037 |
| 99.99 | 264 308 | 3 | 0.00032 | 0.36 | 0.28 | 0.03 |

### 3.2 2 qubits

Table 29: FMUB-FRLS, 2 qubits, random pure states

| $F_B, \%$ | $N_B$ | $M_B$ | $T_{P,B}$, sec | $T_{E,B}$, sec | $\eta_B$ | $O_B$ |
|---|---|---|---|---|---|---|
| 90 | 519 | 9 | 0.00092 | 0.47 | 0.13 | 0 |
| 99 | 46 413 | 9 | 0.00094 | 0.48 | 0.014 | 0.0027 |
| 99.9 | *1 763 979 | – | – | – | – | – |
| 99.99 | *2 742 326 | – | – | – | – | – |

Table 30: FMUB-FRLS, 2 qubits, random mixed states by partial tracing (rank-2) test

| $F_B, \%$ | $N_B$ | $M_B$ | $T_{P,B}$, sec | $T_{E,B}$, sec | $\eta_B$ | $O_B$ |
|---|---|---|---|---|---|---|
| 90 | 616 | 9 | 0.00094 | 0.47 | 0.35 | 0.0035 |
| 99 | 48 837 | 9 | 0.00091 | 0.48 | 0.051 | 0.00062 |
| 99.9 | *1 765 515 | – | – | – | – | – |
| 99.99 | *2 728 501 | – | – | – | – | – |

Table 31: FMUB-FRLS, 2 qubits, random mixed states by partial tracing (full-rank) test

| $F_B, \%$ | $N_B$ | $M_B$ | $T_{P,B}$, sec | $T_{E,B}$, sec | $\eta_B$ | $O_B$ |
|---|---|---|---|---|---|---|
| 90 | *341 | – | – | – | – | – |
| 99 | 15 829 | 9 | 0.00093 | 0.46 | 0.32 | 0.026 |
| 99.9 | 262 741 | 9 | 0.00091 | 0.46 | 0.23 | 0.057 |
| 99.99 | 3 555 013 | 9 | 0.0009 | 0.46 | 0.18 | 0.075 |

Table 32: FMUB-FRLS, 2 qubits, random noisy preparation

| $F_B, \%$ | $N_B$ | $M_B$ | $T_{P,B}$, sec | $T_{E,B}$, sec | $\eta_B$ | $O_B$ |
|---|---|---|---|---|---|---|
| 90 | *160 | – | – | – | – | – |
| 99 | 36 378 | 9 | 0.0011 | 0.68 | 0.11 | 0.01 |
| 99.9 | 1 382 130 | 9 | 0.0011 | 0.66 | 0.05 | 0.038 |
| 99.99 | *10 773 223 | – | – | – | – | – |

### 3.3 3 qubits

Table 33: FMUB-FRLS, 3 qubits, random pure states

| $F_B, \%$ | $N_B$ | $M_B$ | $T_{P,B}$, sec | $T_{E,B}$, sec | $\eta_B$ | $O_B$ |
|---|---|---|---|---|---|---|
| 90 | 1 574 | 27 | 0.002 | 0.53 | 0.073 | 0.0048 |
| 99 | 150 722 | 27 | 0.0021 | 0.54 | 0.0077 | 0.0075 |
| 99.9 | *2 178 934 | – | – | – | – | – |
| 99.99 | *2 785 292 | – | – | – | – | – |

Table 34: FMUB-FRLS, 3 qubits, random mixed states by partial tracing (rank-2) test

| $F_B, \%$ | $N_B$ | $M_B$ | $T_{P,B}$, sec | $T_{E,B}$, sec | $\eta_B$ | $O_B$ |
|---|---|---|---|---|---|---|
| 90 | 2 965 | 27 | 0.0019 | 0.47 | 0.14 | 0.0091 |
| 99 | 276 815 | 27 | 0.0019 | 0.48 | 0.015 | 0.0031 |
| 99.9 | *15 353 412 | – | – | – | – | – |
| 99.99 | *27 097 716 | – | – | – | – | – |

Table 35: FMUB-FRLS, 3 qubits, random mixed states by partial tracing (full-rank) test

| $F_B, \%$ | $N_B$ | $M_B$ | $T_{P,B}$, sec | $T_{E,B}$, sec | $\eta_B$ | $O_B$ |
|---|---|---|---|---|---|---|
| 90 | *1 299 | – | – | – | – | – |
| 99 | 108 665 | 27 | 0.0023 | 0.56 | 0.22 | 0.0072 |
| 99.9 | 2 398 406 | 27 | 0.0022 | 0.57 | 0.15 | 0.048 |
| 99.99 | 40 924 384 | 27 | 0.0022 | 0.56 | 0.11 | 0.067 |

Table 36: FMUB-FRLS, 3 qubits, random noisy preparation

| $F_B, \%$ | $N_B$ | $M_B$ | $T_{P,B}$, sec | $T_{E,B}$, sec | $\eta_B$ | $O_B$ |
|---|---|---|---|---|---|---|
| 90 | *975 | – | – | – | – | – |
| 99 | 317 195 | 27 | 0.0026 | 0.63 | 0.065 | 0.019 |
| 99.9 | 22 250 404 | 27 | 0.0025 | 0.62 | 0.014 | 0.01 |
| 99.99 | *152 226 642 | – | – | – | – | – |

# 4 FMUB-FRML

- Protocol: factorized mutually unbiased bases
- Estimator: full-rank maximum likelihood
- Algorithm: full-rank root approach estimator using [8]
- Machine: Intel(R) Core(TM) i5-7200U CPU @ 2.50GHz

## 4.1 1 qubit

Table 37: FMUB-FRML, 1 qubit, random pure states

| $F_B, \%$ | $N_B$ | $M_B$ | $T_{P,B}$, sec | $T_{E,B}$, sec | $\eta_B$ | $O_B$ |
|---|---|---|---|---|---|---|
| 90 | *83 | – | – | – | – | – |
| 99 | 9 881 | 3 | 0.00041 | 0.0037 | 0.045 | 0 |
| 99.9 | 867 389 | 3 | 0.00036 | 0.0036 | 0.005 | 0 |
| 99.99 | *2 589 235 | – | – | – | – | – |

Table 38: FMUB-FRML, 1 qubit, random mixed states by partial tracing (rank-2) test

| $F_B, \%$ | $N_B$ | $M_B$ | $T_{P,B}$, sec | $T_{E,B}$, sec | $\eta_B$ | $O_B$ |
|---|---|---|---|---|---|---|
| 90 | *48 | – | – | – | – | – |
| 99 | 1 109 | 3 | 0.00044 | 0.0039 | 0.65 | 0.03 |
| 99.9 | 10 126 | 3 | 0.00046 | 0.0039 | 0.62 | 0.037 |
| 99.99 | 106 277 | 3 | 0.00043 | 0.0039 | 0.5 | 0.037 |

Table 39: FMUB-FRML, 1 qubit, random mixed states by partial tracing (full-rank) test

| $F_B, \%$ | $N_B$ | $M_B$ | $T_{P,B}$, sec | $T_{E,B}$, sec | $\eta_B$ | $O_B$ |
|---|---|---|---|---|---|---|
| 90 | *62 | – | – | – | – | – |
| 99 | 994 | 3 | 0.00031 | 0.003 | 0.67 | 0.028 |
| 99.9 | 11 637 | 3 | 0.00031 | 0.0029 | 0.58 | 0.033 |
| 99.99 | 134 940 | 3 | 0.00029 | 0.0029 | 0.42 | 0.046 |

Table 40: FMUB-FRML, 1 qubit, random noisy preparation

| $F_B, \%$ | $N_B$ | $M_B$ | $T_{P,B}$, sec | $T_{E,B}$, sec | $\eta_B$ | $O_B$ |
|---|---|---|---|---|---|---|
| 90 | *19 | – | – | – | – | – |
| 99 | 2 252 | 3 | 0.00033 | 0.0029 | 0.38 | 0.017 |
| 99.9 | 27 014 | 3 | 0.00033 | 0.0029 | 0.3 | 0.037 |
| 99.99 | 264 308 | 3 | 0.00033 | 0.0029 | 0.28 | 0.03 |

### 4.2 2 qubits

Table 41: FMUB-FRML, 2 qubits, random pure states

| $F_B, \%$ | $N_B$ | $M_B$ | $T_{P,B}$, sec | $T_{E,B}$, sec | $\eta_B$ | $O_B$ |
|---|---|---|---|---|---|---|
| 90 | 321 | 9 | 0.00094 | 0.034 | 0.22 | 0.0025 |
| 99 | 23 990 | 9 | 0.00094 | 0.15 | 0.029 | 0.0035 |
| 99.9 | *1 424 621 | – | – | – | – | – |
| 99.99 | *2 655 567 | – | – | – | – | – |

Table 42: FMUB-FRML, 2 qubits, random mixed states by partial tracing (rank-2) test

| $F_B, \%$ | $N_B$ | $M_B$ | $T_{P,B}$, sec | $T_{E,B}$, sec | $\eta_B$ | $O_B$ |
|---|---|---|---|---|---|---|
| 90 | 510 | 9 | 0.00055 | 0.047 | 0.43 | 0.0035 |
| 99 | 36 915 | 9 | 0.00056 | 0.23 | 0.069 | 0.0011 |
| 99.9 | *1 612 140 | – | – | – | – | – |
| 99.99 | *2 716 723 | – | – | – | – | – |

Table 43: FMUB-FRML, 2 qubits, random mixed states by partial tracing (full-rank) test

| $F_B, \%$ | $N_B$ | $M_B$ | $T_{P,B}$, sec | $T_{E,B}$, sec | $\eta_B$ | $O_B$ |
|---|---|---|---|---|---|---|
| 90 | *291 | – | – | – | – | – |
| 99 | 14 593 | 9 | 0.0007 | 0.067 | 0.34 | 0.03 |
| 99.9 | 233 051 | 9 | 0.00067 | 0.068 | 0.25 | 0.069 |
| 99.99 | 3 049 758 | 9 | 0.00068 | 0.073 | 0.2 | 0.084 |

Table 44: FMUB-FRML, 2 qubits, random noisy preparation

| $F_B,\%$ | $N_B$ | $M_B$ | $T_{P,B}$, sec | $T_{E,B}$, sec | $\eta_B$ | $O_B$ |
|---|---|---|---|---|---|---|
| 90 | *128 | – | – | – | – | – |
| 99 | 29 332 | 9 | 0.00053 | 0.14 | 0.13 | 0.012 |
| 99.9 | 1 251 861 | 9 | 0.00051 | 0.18 | 0.06 | 0.039 |
| 99.99 | *10 010 497 | – | – | – | – | – |

### 4.3 3 qubits

Table 45: FMUB-FRML, 3 qubits, random pure states

| $F_B,\%$ | $N_B$ | $M_B$ | $T_{P,B}$, sec | $T_{E,B}$, sec | $\eta_B$ | $O_B$ |
|---|---|---|---|---|---|---|
| 90 | 713 | 27 | 0.0021 | 0.25 | 0.17 | 0.0083 |
| 99 | 48 133 | 27 | 0.0022 | 1.1 | 0.025 | 0.0054 |
| 99.9 | *1 791 982 | – | – | – | – | – |
| 99.99 | *2 788 524 | – | – | – | – | – |

Table 46: FMUB-FRML, 3 qubits, random mixed states by partial tracing (rank-2) test

| $F_B,\%$ | $N_B$ | $M_B$ | $T_{P,B}$, sec | $T_{E,B}$, sec | $\eta_B$ | $O_B$ |
|---|---|---|---|---|---|---|
| 90 | 1 947 | 27 | 0.0018 | 0.4 | 0.21 | 0.012 |
| 99 | 161 345 | 27 | 0.0018 | 1.7 | 0.026 | 0.0093 |
| 99.9 | *12 704 198 | – | – | – | – | – |
| 99.99 | *26 555 178 | – | – | – | – | – |

Table 47: FMUB-FRML, 3 qubits, random mixed states by partial tracing (full-rank) test

| $F_B,\%$ | $N_B$ | $M_B$ | $T_{P,B}$, sec | $T_{E,B}$, sec | $\eta_B$ | $O_B$ |
|---|---|---|---|---|---|---|
| 90 | *1 170 | – | – | – | – | – |
| 99 | 105 039 | 27 | 0.0013 | 0.7 | 0.23 | 0.0072 |
| 99.9 | 2 391 759 | 27 | 0.0013 | 1.2 | 0.16 | 0.032 |
| 99.99 | 38 348 155 | 27 | 0.0013 | 1 | 0.12 | 0.076 |

Table 48: FMUB-FRML, 3 qubits, random noisy preparation

| $F_B,\%$ | $N_B$ | $M_B$ | $T_{P,B}$, sec | $T_{E,B}$, sec | $\eta_B$ | $O_B$ |
|---|---|---|---|---|---|---|
| 90 | *423 | – | – | – | – | – |
| 99 | 215 852 | 27 | 0.0014 | 1.1 | 0.095 | 0.018 |
| 99.9 | 18 382 472 | 27 | 0.0013 | 2 | 0.019 | 0.016 |
| 99.99 | *145 112 112 | – | – | – | – | – |

## 5 FMUB-TRML

- Protocol: factorized mutually unbiased bases

- Estimator: true-rank maximum likelihood
- Algorithm: true-rank root approach estimator using [8]
- Parameters: a-priori known density matrix rank $r$
- Machine: Intel(R) Core(TM) i5-7200U CPU @ 2.50GHz

### 5.1 1 qubit

Table 49: FMUB-TRML, 1 qubit, random pure states

| $F_B, \%$ | $N_B$ | $M_B$ | $T_{P,B}$, sec | $T_{E,B}$, sec | $\eta_B$ | $O_B$ |
|---|---|---|---|---|---|---|
| 90 | *1 | – | – | – | – | – |
| 99 | 339 | 3 | 0.00052 | 0.0058 | 0.91 | 0.0064 |
| 99.9 | 3 387 | 3 | 0.00053 | 0.0059 | 0.9 | 0.004 |
| 99.99 | 32 859 | 3 | 0.00055 | 0.0055 | 0.92 | 0.0061 |

Table 50: FMUB-TRML, 1 qubit, random mixed states by partial tracing (rank-2) test

| $F_B, \%$ | $N_B$ | $M_B$ | $T_{P,B}$, sec | $T_{E,B}$, sec | $\eta_B$ | $O_B$ |
|---|---|---|---|---|---|---|
| 90 | *48 | – | – | – | – | – |
| 99 | 1 109 | 3 | 0.00043 | 0.0047 | 0.65 | 0.03 |
| 99.9 | 10 126 | 3 | 0.00045 | 0.0049 | 0.62 | 0.037 |
| 99.99 | 106 277 | 3 | 0.0005 | 0.005 | 0.5 | 0.037 |

Table 51: FMUB-TRML, 1 qubit, random mixed states by partial tracing (full-rank) test

| $F_B, \%$ | $N_B$ | $M_B$ | $T_{P,B}$, sec | $T_{E,B}$, sec | $\eta_B$ | $O_B$ |
|---|---|---|---|---|---|---|
| 90 | *62 | – | – | – | – | – |
| 99 | 994 | 3 | 0.00031 | 0.003 | 0.67 | 0.028 |
| 99.9 | 11 637 | 3 | 0.00031 | 0.0029 | 0.58 | 0.033 |
| 99.99 | 134 940 | 3 | 0.00029 | 0.0029 | 0.42 | 0.046 |

Table 52: FMUB-TRML, 1 qubit, random noisy preparation

| $F_B, \%$ | $N_B$ | $M_B$ | $T_{P,B}$, sec | $T_{E,B}$, sec | $\eta_B$ | $O_B$ |
|---|---|---|---|---|---|---|
| 90 | *19 | – | – | – | – | – |
| 99 | 2 252 | 3 | 0.00033 | 0.0029 | 0.38 | 0.017 |
| 99.9 | 27 014 | 3 | 0.00033 | 0.0029 | 0.3 | 0.037 |
| 99.99 | 264 308 | 3 | 0.00033 | 0.0029 | 0.28 | 0.03 |

### 5.2 2 qubits

Table 53: FMUB-TRML, 2 qubits, random pure states

| $F_B, \%$ | $N_B$ | $M_B$ | $T_{P,B}$, sec | $T_{E,B}$, sec | $\eta_B$ | $O_B$ |
|---|---|---|---|---|---|---|
| 90 | *63 | – | – | – | – | – |
| 99 | 750 | 9 | 0.0013 | 0.0079 | 0.89 | 0.024 |
| 99.9 | 7 205 | 9 | 0.0014 | 0.0081 | 0.9 | 0.0098 |
| 99.99 | 70 588 | 9 | 0.0013 | 0.0077 | 0.92 | 0.0045 |

Table 54: FMUB-TRML, 2 qubits, random mixed states by partial tracing (rank-2) test

| $F_B, \%$ | $N_B$ | $M_B$ | $T_{P,B}$, sec | $T_{E,B}$, sec | $\eta_B$ | $O_B$ |
|---|---|---|---|---|---|---|
| 90 | 285 | 9 | 0.00087 | 0.011 | 0.72 | 0.03 |
| 99 | 3 367 | 9 | 0.00086 | 0.011 | 0.61 | 0.026 |
| 99.9 | 33 783 | 9 | 0.00086 | 0.0092 | 0.62 | 0.022 |
| 99.99 | 340 894 | 9 | 0.00086 | 0.0085 | 0.62 | 0.022 |

Table 55: FMUB-TRML, 2 qubits, random mixed states by partial tracing (full-rank) test

| $F_B, \%$ | $N_B$ | $M_B$ | $T_{P,B}$, sec | $T_{E,B}$, sec | $\eta_B$ | $O_B$ |
|---|---|---|---|---|---|---|
| 90 | *291 | – | – | – | – | – |
| 99 | 14 593 | 9 | 0.0007 | 0.067 | 0.34 | 0.03 |
| 99.9 | 233 051 | 9 | 0.00067 | 0.068 | 0.25 | 0.069 |
| 99.99 | 3 049 758 | 9 | 0.00068 | 0.073 | 0.2 | 0.084 |

Table 56: FMUB-TRML, 2 qubits, random noisy preparation

| $F_B, \%$ | $N_B$ | $M_B$ | $T_{P,B}$, sec | $T_{E,B}$, sec | $\eta_B$ | $O_B$ |
|---|---|---|---|---|---|---|
| 90 | *128 | – | – | – | – | – |
| 99 | 29 332 | 9 | 0.00053 | 0.14 | 0.13 | 0.012 |
| 99.9 | 1 251 861 | 9 | 0.00051 | 0.18 | 0.06 | 0.039 |
| 99.99 | *10 010 497 | – | – | – | – | – |

### 5.3 3 qubits

Table 57: FMUB-TRML, 3 qubits, random pure states

| $F_B, \%$ | $N_B$ | $M_B$ | $T_{P,B}$, sec | $T_{E,B}$, sec | $\eta_B$ | $O_B$ |
|---|---|---|---|---|---|---|
| 90 | 163 | 27 | 0.002 | 0.014 | 0.81 | 0.019 |
| 99 | 1 380 | 27 | 0.002 | 0.011 | 0.89 | 0.0081 |
| 99.9 | 12 960 | 27 | 0.0021 | 0.011 | 0.92 | 0.015 |
| 99.99 | 133 258 | 27 | 0.0021 | 0.01 | 0.93 | 0.011 |

Table 58: FMUB-TRML, 3 qubits, random mixed states by partial tracing (rank-2) test

| $F_B$, % | $N_B$ | $M_B$ | $T_{P,B}$, sec | $T_{E,B}$, sec | $\eta_B$ | $O_B$ |
|---|---|---|---|---|---|---|
| 90 | *257 | – | – | – | – | – |
| 99 | 6 001 | 27 | 0.003 | 0.031 | 0.71 | 0.011 |
| 99.9 | 57 833 | 27 | 0.0033 | 0.026 | 0.72 | 0.0082 |
| 99.99 | 577 409 | 27 | 0.0031 | 0.025 | 0.72 | 0.012 |

Table 59: FMUB-TRML, 3 qubits, random mixed states by partial tracing (full-rank) test

| $F_B$, % | $N_B$ | $M_B$ | $T_{P,B}$, sec | $T_{E,B}$, sec | $\eta_B$ | $O_B$ |
|---|---|---|---|---|---|---|
| 90 | *1 170 | – | – | – | – | – |
| 99 | 105 039 | 27 | 0.0013 | 0.7 | 0.23 | 0.0072 |
| 99.9 | 2 391 759 | 27 | 0.0013 | 1.2 | 0.16 | 0.032 |
| 99.99 | 38 348 155 | 27 | 0.0013 | 1 | 0.12 | 0.076 |

Table 60: FMUB-TRML, 3 qubits, random noisy preparation

| $F_B$, % | $N_B$ | $M_B$ | $T_{P,B}$, sec | $T_{E,B}$, sec | $\eta_B$ | $O_B$ |
|---|---|---|---|---|---|---|
| 90 | *423 | – | – | – | – | – |
| 99 | 215 852 | 27 | 0.0014 | 1.1 | 0.095 | 0.018 |
| 99.9 | 18 382 472 | 27 | 0.0013 | 2 | 0.019 | 0.016 |
| 99.99 | *145 112 112 | – | – | – | – | – |

# 6 FMUB-ARML

- Protocol: factorized mutually unbiased bases
- Estimator: adequate rank maximum likelihood
- Algorithm: adequate rank root approach estimator using [8]
- Parameters: significance level 5%
- Machine: Intel(R) Core(TM) i5-7200U CPU @ 2.50GHz

## 6.1 1 qubit

Table 61: FMUB-ARML, 1 qubit, random pure states

| $F_B$, % | $N_B$ | $M_B$ | $T_{P,B}$, sec | $T_{E,B}$, sec | $\eta_B$ | $O_B$ |
|---|---|---|---|---|---|---|
| 90 | *1 | – | – | – | – | – |
| 99 | 381 | 3 | 0.00069 | 0.009 | 0.63 | 0.02 |
| 99.9 | 4 429 | 3 | 0.00071 | 0.0088 | 0.28 | 0.027 |
| 99.99 | 43 310 | 3 | 0.00065 | 0.0088 | 0.12 | 0.029 |

Table 62: FMUB-ARML, 1 qubit, random mixed states by partial tracing (rank-2) test

| $F_B, \%$ | $N_B$ | $M_B$ | $T_{P,B}$, sec | $T_{E,B}$, sec | $\eta_B$ | $O_B$ |
|---:|---:|---:|---:|---:|---:|---:|
| 90 | 214 | 3 | 0.00073 | 0.013 | 0.37 | 0.042 |
| 99 | 2 735 | 3 | 0.00071 | 0.022 | 0.34 | 0.096 |
| 99.9 | 18 008 | 3 | 0.00072 | 0.037 | 0.32 | 0.052 |
| 99.99 | 114 501 | 3 | 0.00069 | 0.049 | 0.3 | 0.042 |

Table 63: FMUB-ARML, 1 qubit, random mixed states by partial tracing (full-rank) test

| $F_B, \%$ | $N_B$ | $M_B$ | $T_{P,B}$, sec | $T_{E,B}$, sec | $\eta_B$ | $O_B$ |
|---:|---:|---:|---:|---:|---:|---:|
| 90 | 225 | 3 | 0.00051 | 0.0094 | 0.37 | 0.039 |
| 99 | 2 739 | 3 | 0.0005 | 0.017 | 0.33 | 0.089 |
| 99.9 | 19 430 | 3 | 0.00053 | 0.029 | 0.31 | 0.058 |
| 99.99 | 160 823 | 3 | 0.00054 | 0.035 | 0.28 | 0.051 |

Table 64: FMUB-ARML, 1 qubit, random noisy preparation

| $F_B, \%$ | $N_B$ | $M_B$ | $T_{P,B}$, sec | $T_{E,B}$, sec | $\eta_B$ | $O_B$ |
|---:|---:|---:|---:|---:|---:|---:|
| 90 | *18 | – | – | – | – | – |
| 99 | 10 520 | 3 | 0.00049 | 0.0084 | 0.12 | 0.1 |
| 99.9 | 50 048 | 3 | 0.00048 | 0.0098 | 0.12 | 0.067 |
| 99.99 | 318 920 | 3 | 0.00046 | 0.02 | 0.16 | 0.039 |

## 6.2 2 qubits

Table 65: FMUB-ARML, 2 qubits, random pure states

| $F_B, \%$ | $N_B$ | $M_B$ | $T_{P,B}$, sec | $T_{E,B}$, sec | $\eta_B$ | $O_B$ |
|---:|---:|---:|---:|---:|---:|---:|
| 90 | *89 | – | – | – | – | – |
| 99 | 801 | 9 | 0.0014 | 0.013 | 0.68 | 0.054 |
| 99.9 | 7 798 | 9 | 0.0014 | 0.013 | 0.57 | 0.022 |
| 99.99 | 75 357 | 9 | 0.0014 | 0.011 | 0.36 | 0.014 |

Table 66: FMUB-ARML, 2 qubits, random mixed states by partial tracing (rank-2) test

| $F_B, \%$ | $N_B$ | $M_B$ | $T_{P,B}$, sec | $T_{E,B}$, sec | $\eta_B$ | $O_B$ |
|---:|---:|---:|---:|---:|---:|---:|
| 90 | 399 | 9 | 0.0011 | 0.022 | 0.55 | 0.023 |
| 99 | 3 856 | 9 | 0.0011 | 0.037 | 0.55 | 0.037 |
| 99.9 | 37 554 | 9 | 0.0011 | 0.057 | 0.46 | 0.037 |
| 99.99 | 378 165 | 9 | 0.0012 | 0.063 | 0.29 | 0.034 |

Table 67: FMUB-ARML, 2 qubits, random mixed states by partial tracing (full-rank) test

| $F_B, \%$ | $N_B$ | $M_B$ | $T_{P,B}$, sec | $T_{E,B}$, sec | $\eta_B$ | $O_B$ |
|---:|---:|---:|---:|---:|---:|---:|
| 90 | 2 013 | 9 | 0.0012 | 0.058 | 0.21 | 0 |
| 99 | 105 060 | 9 | 0.0012 | 0.11 | 0.073 | 0.016 |
| 99.9 | 2 005 212 | 9 | 0.0012 | 0.14 | 0.058 | 0.18 |
| 99.99 | *10 815 451 | – | – | – | – | – |

Table 68: FMUB-ARML, 2 qubits, random noisy preparation

| $F_B, \%$ | $N_B$ | $M_B$ | $T_{P,B}$, sec | $T_{E,B}$, sec | $\eta_B$ | $O_B$ |
|---:|---:|---:|---:|---:|---:|---:|
| 90 | *409 | – | – | – | – | – |
| 99 | 138 057 | 9 | 0.0012 | 0.21 | 0.036 | 0.1 |
| 99.9 | 6 238 296 | 9 | 0.0012 | 0.47 | 0.017 | 0.13 |
| 99.99 | *17 458 991 | – | – | – | – | – |

## 6.3 3 qubits

Table 69: FMUB-ARML, 3 qubits, random pure states

| $F_B, \%$ | $N_B$ | $M_B$ | $T_{P,B}$, sec | $T_{E,B}$, sec | $\eta_B$ | $O_B$ |
|---:|---:|---:|---:|---:|---:|---:|
| 90 | 167 | 27 | 0.0018 | 0.015 | 0.77 | 0.027 |
| 99 | 1 565 | 27 | 0.0019 | 0.016 | 0.68 | 0.036 |
| 99.9 | 15 381 | 27 | 0.0018 | 0.037 | 0.5 | 0.039 |
| 99.99 | 143 532 | 27 | 0.0019 | 0.13 | 0.34 | 0.031 |

Table 70: FMUB-ARML, 3 qubits, random mixed states by partial tracing (rank-2) test

| $F_B, \%$ | $N_B$ | $M_B$ | $T_{P,B}$, sec | $T_{E,B}$, sec | $\eta_B$ | $O_B$ |
|---:|---:|---:|---:|---:|---:|---:|
| 90 | *386 | – | – | – | – | – |
| 99 | 6 450 | 27 | 0.0019 | 0.062 | 0.64 | 0.023 |
| 99.9 | 60 677 | 27 | 0.0019 | 0.066 | 0.52 | 0.021 |
| 99.99 | 602 455 | 27 | 0.0018 | 0.059 | 0.38 | 0.023 |

Table 71: FMUB-ARML, 3 qubits, random mixed states by partial tracing (full-rank) test

| $F_B, \%$ | $N_B$ | $M_B$ | $T_{P,B}$, sec | $T_{E,B}$, sec | $\eta_B$ | $O_B$ |
|---:|---:|---:|---:|---:|---:|---:|
| 90 | 19 160 | 27 | 0.0028 | 0.78 | 0.12 | 0.0044 |
| 99 | 646 936 | 27 | 0.0025 | 1.2 | 0.055 | 0.0015 |
| 99.9 | 36 526 642 | 27 | 0.0026 | 1.4 | 0.019 | 0.099 |
| 99.99 | *227 858 692 | – | – | – | – | – |

Table 72: FMUB-ARML, 3 qubits, random noisy preparation

| $F_B, \%$ | $N_B$ | $M_B$ | $T_{P,B}$, sec | $T_{E,B}$, sec | $\eta_B$ | $O_B$ |
|---:|---:|---:|---:|---:|---:|---:|
| 90 | *9 197 | – | – | – | – | – |
| 99 | 908 286 | 27 | 0.0023 | 2 | 0.025 | 0.022 |
| 99.9 | *104 503 809 | – | – | – | – | – |
| 99.99 | *208 389 099 | – | – | – | – | – |

# 7 FMUB-CS

- Protocol: factorized mutually unbiased bases
- Estimator: compressed sensing [1]
- Algorithm: convex density matrix trace minimization using [7]
- Parameters: $\varepsilon = \hat{\varepsilon}(1+\alpha)$ ($\alpha$ is varying from 0 with step 0.1 till problem becomes feasible)
- Machine: Intel(R) Core(TM) i5-7200U CPU @ 2.50GHz

## 7.1 1 qubit

Table 73: FMUB-CS, 1 qubit, random pure states

| $F_B, \%$ | $N_B$ | $M_B$ | $T_{P,B}$, sec | $T_{E,B}$, sec | $\eta_B$ | $O_B$ |
|---:|---:|---:|---:|---:|---:|---:|
| 90 | *2 | – | – | – | – | – |
| 99 | 599 | 3 | 0.00034 | 0.47 | 0.56 | 0.023 |
| 99.9 | 56 212 | 3 | 0.00034 | 0.44 | 0.11 | 0.11 |
| 99.99 | *1 811 808 | – | – | – | – | – |

Table 74: FMUB-CS, 1 qubit, random mixed states by partial tracing (rank-2) test

| $F_B, \%$ | $N_B$ | $M_B$ | $T_{P,B}$, sec | $T_{E,B}$, sec | $\eta_B$ | $O_B$ |
|---:|---:|---:|---:|---:|---:|---:|
| 90 | 158 | 3 | 0.00044 | 0.59 | 0.41 | 0.012 |
| 99 | 2 936 | 3 | 0.00042 | 0.58 | 0.31 | 0.057 |
| 99.9 | 31 718 | 3 | 0.00042 | 0.58 | 0.26 | 0.05 |
| 99.99 | 281 587 | 3 | 0.0004 | 0.59 | 0.24 | 0.042 |

Table 75: FMUB-CS, 1 qubit, random mixed states by partial tracing (full-rank) test

| $F_B, \%$ | $N_B$ | $M_B$ | $T_{P,B}$, sec | $T_{E,B}$, sec | $\eta_B$ | $O_B$ |
|---:|---:|---:|---:|---:|---:|---:|
| 90 | 165 | 3 | 0.00036 | 0.52 | 0.4 | 0.012 |
| 99 | 2 758 | 3 | 0.00037 | 0.5 | 0.31 | 0.069 |
| 99.9 | 31 857 | 3 | 0.00038 | 0.49 | 0.25 | 0.07 |
| 99.99 | 327 330 | 3 | 0.00037 | 0.5 | 0.2 | 0.053 |

Table 76: FMUB-CS, 1 qubit, random noisy preparation

| $F_B, \%$ | $N_B$ | $M_B$ | $T_{P,B}$, sec | $T_{E,B}$, sec | $\eta_B$ | $O_B$ |
|---|---|---|---|---|---|---|
| 90 | *15 | – | – | – | – | – |
| 99 | 6 733 | 3 | 0.00042 | 0.53 | 0.13 | 0.0066 |
| 99.9 | 84 784 | 3 | 0.00039 | 0.52 | 0.1 | 0.061 |
| 99.99 | 704 194 | 3 | 0.0004 | 0.53 | 0.11 | 0.066 |

## 7.2 2 qubits

Table 77: FMUB-CS, 2 qubits, random pure states

| $F_B, \%$ | $N_B$ | $M_B$ | $T_{P,B}$, sec | $T_{E,B}$, sec | $\eta_B$ | $O_B$ |
|---|---|---|---|---|---|---|
| 90 | 220 | 9 | 0.0008 | 1 | 0.37 | 0.029 |
| 99 | 13 959 | 9 | 0.00084 | 0.76 | 0.092 | 0.037 |
| 99.9 | *1 123 593 | – | – | – | – | – |
| 99.99 | *2 710 677 | – | – | – | – | – |

Table 78: FMUB-CS, 2 qubits, random mixed states by partial tracing (rank-2) test

| $F_B, \%$ | $N_B$ | $M_B$ | $T_{P,B}$, sec | $T_{E,B}$, sec | $\eta_B$ | $O_B$ |
|---|---|---|---|---|---|---|
| 90 | 411 | 9 | 0.00083 | 0.59 | 0.52 | 0.017 |
| 99 | 17 178 | 9 | 0.00087 | 0.44 | 0.2 | 0.06 |
| 99.9 | *1 156 881 | – | – | – | – | – |
| 99.99 | *2 334 153 | – | – | – | – | – |

Table 79: FMUB-CS, 2 qubits, random mixed states by partial tracing (full-rank) test

| $F_B, \%$ | $N_B$ | $M_B$ | $T_{P,B}$, sec | $T_{E,B}$, sec | $\eta_B$ | $O_B$ |
|---|---|---|---|---|---|---|
| 90 | *759 | – | – | – | – | – |
| 99 | 28 781 | 9 | 0.00092 | 0.53 | 0.19 | 0.03 |
| 99.9 | 572 506 | 9 | 0.00092 | 0.52 | 0.13 | 0.091 |
| 99.99 | 8 325 077 | 9 | 0.00094 | 0.53 | 0.087 | 0.1 |

Table 80: FMUB-CS, 2 qubits, random noisy preparation

| $F_B, \%$ | $N_B$ | $M_B$ | $T_{P,B}$, sec | $T_{E,B}$, sec | $\eta_B$ | $O_B$ |
|---|---|---|---|---|---|---|
| 90 | *196 | – | – | – | – | – |
| 99 | 51 776 | 9 | 0.00087 | 0.5 | 0.07 | 0.016 |
| 99.9 | 2 234 214 | 9 | 0.00091 | 0.49 | 0.027 | 0.014 |
| 99.99 | *12 042 970 | – | – | – | – | – |

### 7.3 3 qubits

Table 81: FMUB-CS, 3 qubits, random pure states

| $F_B, \%$ | $N_B$ | $M_B$ | $T_{P,B}$, sec | $T_{E,B}$, sec | $\eta_B$ | $O_B$ |
|---|---|---|---|---|---|---|
| 90 | 751 | 27 | 0.0018 | 0.87 | 0.22 | 0.0028 |
| 99 | 47 889 | 27 | 0.0019 | 0.77 | 0.046 | 0.00068 |
| 99.9 | *2 187 271 | – | – | – | – | – |
| 99.99 | *3 551 649 | – | – | – | – | – |

Table 82: FMUB-CS, 3 qubits, random mixed states by partial tracing (rank-2) test

| $F_B, \%$ | $N_B$ | $M_B$ | $T_{P,B}$, sec | $T_{E,B}$, sec | $\eta_B$ | $O_B$ |
|---|---|---|---|---|---|---|
| 90 | 1 648 | 27 | 0.002 | 0.71 | 0.3 | 0.0034 |
| 99 | 97 437 | 27 | 0.002 | 0.52 | 0.062 | 0.0099 |
| 99.9 | 9 445 112 | 27 | 0.0019 | 0.55 | 0.0068 | 0.003 |
| 99.99 | *25 562 993 | – | – | – | – | – |

Table 83: FMUB-CS, 3 qubits, random mixed states by partial tracing (full-rank) test

| $F_B, \%$ | $N_B$ | $M_B$ | $T_{P,B}$, sec | $T_{E,B}$, sec | $\eta_B$ | $O_B$ |
|---|---|---|---|---|---|---|
| 90 | *2 331 | – | – | – | – | – |
| 99 | 144 109 | 27 | 0.0027 | 0.57 | 0.17 | 0.0072 |
| 99.9 | 3 733 351 | 27 | 0.0026 | 0.58 | 0.1 | 0.043 |
| 99.99 | 70 297 469 | 27 | 0.0027 | 0.63 | 0.074 | 0.091 |

Table 84: FMUB-CS, 3 qubits, random noisy preparation

| $F_B, \%$ | $N_B$ | $M_B$ | $T_{P,B}$, sec | $T_{E,B}$, sec | $\eta_B$ | $O_B$ |
|---|---|---|---|---|---|---|
| 90 | *1 295 | – | – | – | – | – |
| 99 | 351 892 | 27 | 0.0037 | 0.87 | 0.06 | 0.018 |
| 99.9 | 29 173 307 | 27 | 0.0039 | 0.91 | 0.011 | 0.0083 |
| 99.99 | *160 348 622 | – | – | – | – | – |

# 8 Pauli-CS

- Protocol: factorized Pauli observables measurements
- Estimator: compressed sensing [2]
- Algorithm: convex density matrix trace minimization using [7]
- Parameters: lasso estimator, $\mu = 4m/\sqrt{N}$
- Machine: Intel(R) Core(TM) i5-7200U CPU @ 2.50GHz

### 8.1 1 qubit

Table 85: FMUB-CS, 1 qubit, random pure states

| $F_B, \%$ | $N_B$ | $M_B$ | $T_{P,B}$, sec | $T_{E,B}$, sec | $\eta_B$ | $O_B$ |
|---|---|---|---|---|---|---|
| 90 | *2 | – | – | – | – | – |
| 99 | 599 | 3 | 0.00034 | 0.47 | 0.56 | 0.023 |
| 99.9 | 56 212 | 3 | 0.00034 | 0.44 | 0.11 | 0.11 |
| 99.99 | *1 811 808 | – | – | – | – | – |

Table 86: FMUB-CS, 1 qubit, random mixed states by partial tracing (rank-2) test

| $F_B, \%$ | $N_B$ | $M_B$ | $T_{P,B}$, sec | $T_{E,B}$, sec | $\eta_B$ | $O_B$ |
|---|---|---|---|---|---|---|
| 90 | 158 | 3 | 0.00044 | 0.59 | 0.41 | 0.012 |
| 99 | 2 936 | 3 | 0.00042 | 0.58 | 0.31 | 0.057 |
| 99.9 | 31 718 | 3 | 0.00042 | 0.58 | 0.26 | 0.05 |
| 99.99 | 281 587 | 3 | 0.0004 | 0.59 | 0.24 | 0.042 |

Table 87: FMUB-CS, 1 qubit, random mixed states by partial tracing (full-rank) test

| $F_B, \%$ | $N_B$ | $M_B$ | $T_{P,B}$, sec | $T_{E,B}$, sec | $\eta_B$ | $O_B$ |
|---|---|---|---|---|---|---|
| 90 | 165 | 3 | 0.00036 | 0.52 | 0.4 | 0.012 |
| 99 | 2 758 | 3 | 0.00037 | 0.5 | 0.31 | 0.069 |
| 99.9 | 31 857 | 3 | 0.00038 | 0.49 | 0.25 | 0.07 |
| 99.99 | 327 330 | 3 | 0.00037 | 0.5 | 0.2 | 0.053 |

Table 88: FMUB-CS, 1 qubit, random noisy preparation

| $F_B, \%$ | $N_B$ | $M_B$ | $T_{P,B}$, sec | $T_{E,B}$, sec | $\eta_B$ | $O_B$ |
|---|---|---|---|---|---|---|
| 90 | *15 | – | – | – | – | – |
| 99 | 6 733 | 3 | 0.00042 | 0.53 | 0.13 | 0.0066 |
| 99.9 | 84 784 | 3 | 0.00039 | 0.52 | 0.1 | 0.061 |
| 99.99 | 704 194 | 3 | 0.0004 | 0.53 | 0.11 | 0.066 |

### 8.2 2 qubits

Table 89: FMUB-CS, 2 qubits, random pure states

| $F_B, \%$ | $N_B$ | $M_B$ | $T_{P,B}$, sec | $T_{E,B}$, sec | $\eta_B$ | $O_B$ |
|---|---|---|---|---|---|---|
| 90 | 220 | 9 | 0.0008 | 1 | 0.37 | 0.029 |
| 99 | 13 959 | 9 | 0.00084 | 0.76 | 0.092 | 0.037 |
| 99.9 | *1 123 593 | – | – | – | – | – |
| 99.99 | *2 710 677 | – | – | – | – | – |

Table 90: FMUB-CS, 2 qubits, random mixed states by partial tracing (rank-2) test

| $F_B, \%$ | $N_B$ | $M_B$ | $T_{P,B}$, sec | $T_{E,B}$, sec | $\eta_B$ | $O_B$ |
|---|---|---|---|---|---|---|
| 90 | 411 | 9 | 0.00083 | 0.59 | 0.52 | 0.017 |
| 99 | 17 178 | 9 | 0.00087 | 0.44 | 0.2 | 0.06 |
| 99.9 | *1 156 881 | – | – | – | – | – |
| 99.99 | *2 334 153 | – | – | – | – | – |

Table 91: FMUB-CS, 2 qubits, random mixed states by partial tracing (full-rank) test

| $F_B, \%$ | $N_B$ | $M_B$ | $T_{P,B}$, sec | $T_{E,B}$, sec | $\eta_B$ | $O_B$ |
|---|---|---|---|---|---|---|
| 90 | *759 | – | – | – | – | – |
| 99 | 28 781 | 9 | 0.00092 | 0.53 | 0.19 | 0.03 |
| 99.9 | 572 506 | 9 | 0.00092 | 0.52 | 0.13 | 0.091 |
| 99.99 | 8 325 077 | 9 | 0.00094 | 0.53 | 0.087 | 0.1 |

Table 92: FMUB-CS, 2 qubits, random noisy preparation

| $F_B, \%$ | $N_B$ | $M_B$ | $T_{P,B}$, sec | $T_{E,B}$, sec | $\eta_B$ | $O_B$ |
|---|---|---|---|---|---|---|
| 90 | *196 | – | – | – | – | – |
| 99 | 51 776 | 9 | 0.00087 | 0.5 | 0.07 | 0.016 |
| 99.9 | 2 234 214 | 9 | 0.00091 | 0.49 | 0.027 | 0.014 |
| 99.99 | *12 042 970 | – | – | – | – | – |

## 8.3 3 qubits

Table 93: FMUB-CS, 3 qubits, random pure states

| $F_B, \%$ | $N_B$ | $M_B$ | $T_{P,B}$, sec | $T_{E,B}$, sec | $\eta_B$ | $O_B$ |
|---|---|---|---|---|---|---|
| 90 | 751 | 27 | 0.0018 | 0.87 | 0.22 | 0.0028 |
| 99 | 47 889 | 27 | 0.0019 | 0.77 | 0.046 | 0.00068 |
| 99.9 | *2 187 271 | – | – | – | – | – |
| 99.99 | *3 551 649 | – | – | – | – | – |

Table 94: FMUB-CS, 3 qubits, random mixed states by partial tracing (rank-2) test

| $F_B, \%$ | $N_B$ | $M_B$ | $T_{P,B}$, sec | $T_{E,B}$, sec | $\eta_B$ | $O_B$ |
|---|---|---|---|---|---|---|
| 90 | 1 648 | 27 | 0.002 | 0.71 | 0.3 | 0.0034 |
| 99 | 97 437 | 27 | 0.002 | 0.52 | 0.062 | 0.0099 |
| 99.9 | 9 445 112 | 27 | 0.0019 | 0.55 | 0.0068 | 0.003 |
| 99.99 | *25 562 993 | – | – | – | – | – |

Table 95: FMUB-CS, 3 qubits, random mixed states by partial tracing (full-rank) test

| $F_B$, % | $N_B$ | $M_B$ | $T_{P,B}$, sec | $T_{E,B}$, sec | $\eta_B$ | $O_B$ |
|---|---|---|---|---|---|---|
| 90 | *2 331 | – | – | – | – | – |
| 99 | 144 109 | 27 | 0.0027 | 0.57 | 0.17 | 0.0072 |
| 99.9 | 3 733 351 | 27 | 0.0026 | 0.58 | 0.1 | 0.043 |
| 99.99 | 70 297 469 | 27 | 0.0027 | 0.63 | 0.074 | 0.091 |

Table 96: FMUB-CS, 3 qubits, random noisy preparation

| $F_B$, % | $N_B$ | $M_B$ | $T_{P,B}$, sec | $T_{E,B}$, sec | $\eta_B$ | $O_B$ |
|---|---|---|---|---|---|---|
| 90 | *1 295 | – | – | – | – | – |
| 99 | 351 892 | 27 | 0.0037 | 0.87 | 0.06 | 0.018 |
| 99.9 | 29 173 307 | 27 | 0.0039 | 0.91 | 0.011 | 0.0083 |
| 99.99 | *160 348 622 | – | – | – | – | – |

# 9 AMUB-FRML

- Protocol: adaptive mutually unbiased bases
- Estimator: full-rank maximum likelihood
- Algorithm: full-rank root approach estimator using [8]
- Machine: Intel(R) Xeon(R) CPU E5450 @ 3.00GHz

## 9.1 1 qubit

Table 97: AMUB-FRML, 1 qubit, random pure states

| $F_B$, % | $N_B$ | $M_B$ | $T_{P,B}$, sec | $T_{E,B}$, sec | $\eta_B$ | $O_B$ |
|---|---|---|---|---|---|---|
| 90 | *86 | – | – | – | – | – |
| 99 | 990 | 12 | 0.067 | 0.027 | 0.41 | 0.032 |
| 99.9 | 8 802 | 66 | 0.73 | 0.04 | 0.46 | 0.015 |
| 99.99 | 106 287 | 143 | 1.6 | 0.04 | 0.35 | 0.0051 |

Table 98: AMUB-FRML, 1 qubit, random mixed states by partial tracing (rank-2) test

| $F_B$, % | $N_B$ | $M_B$ | $T_{P,B}$, sec | $T_{E,B}$, sec | $\eta_B$ | $O_B$ |
|---|---|---|---|---|---|---|
| 90 | *50 | – | – | – | – | – |
| 99 | 750 | 11 | 0.021 | 0.0087 | 0.85 | 0.017 |
| 99.9 | 6 332 | 58 | 0.2 | 0.013 | 0.97 | 0.0078 |
| 99.99 | 58 516 | 124 | 0.5 | 0.021 | 1 | 0.0027 |

Table 99: AMUB-FRML, 1 qubit, random mixed states by partial tracing (full-rank) test

| $F_B, \%$ | $N_B$ | $M_B$ | $T_{P,B}$, sec | $T_{E,B}$, sec | $\eta_B$ | $O_B$ |
|---|---|---|---|---|---|---|
| 90 | *63 | – | – | – | – | – |
| 99 | 731 | 11 | 0.022 | 0.009 | 0.85 | 0.013 |
| 99.9 | 6 115 | 57 | 0.19 | 0.013 | 0.95 | 0.0095 |
| 99.99 | 60 176 | 125 | 0.51 | 0.017 | 0.99 | 0.0041 |

Table 100: AMUB-FRML, 1 qubit, random noisy preparation

| $F_B, \%$ | $N_B$ | $M_B$ | $T_{P,B}$, sec | $T_{E,B}$, sec | $\eta_B$ | $O_B$ |
|---|---|---|---|---|---|---|
| 90 | *25 | – | – | – | – | – |
| 99 | 1 051 | 13 | 0.042 | 0.012 | 0.72 | 0.029 |
| 99.9 | 6 612 | 59 | 0.21 | 0.014 | 0.93 | 0.012 |
| 99.99 | 62 663 | 126 | 0.53 | 0.021 | 0.96 | 0.0032 |

### 9.2 2 qubits

Table 101: AMUB-FRML, 2 qubits, random pure states

| $F_B, \%$ | $N_B$ | $M_B$ | $T_{P,B}$, sec | $T_{E,B}$, sec | $\eta_B$ | $O_B$ |
|---|---|---|---|---|---|---|
| 90 | 228 | 7 | 0.04 | 0.12 | 0.32 | 0.0026 |
| 99 | 2 632 | 35 | 0.87 | 0.21 | 0.31 | 0.0013 |
| 99.9 | 23 472 | 98 | 2.9 | 0.31 | 0.35 | 0.0026 |
| 99.99 | 229 502 | 172 | 6.2 | 0.33 | 0.37 | 0.015 |

Table 102: AMUB-FRML, 2 qubits, random mixed states by partial tracing (rank-2) test

| $F_B, \%$ | $N_B$ | $M_B$ | $T_{P,B}$, sec | $T_{E,B}$, sec | $\eta_B$ | $O_B$ |
|---|---|---|---|---|---|---|
| 90 | 416 | 8 | 0.07 | 0.089 | 0.52 | 0.0042 |
| 99 | 6 850 | 60 | 1.7 | 0.24 | 0.34 | 0.012 |
| 99.9 | 77 273 | 137 | 6.1 | 0.57 | 0.32 | 0.018 |
| 99.99 | 895 449 | 216 | 13 | 0.92 | 0.29 | 0.013 |

Table 103: AMUB-FRML, 2 qubits, random mixed states by partial tracing (full-rank) test

| $F_B, \%$ | $N_B$ | $M_B$ | $T_{P,B}$, sec | $T_{E,B}$, sec | $\eta_B$ | $O_B$ |
|---|---|---|---|---|---|---|
| 90 | *146 | – | – | – | – | – |
| 99 | 8 842 | 67 | 0.76 | 0.083 | 0.55 | 0.046 |
| 99.9 | 62 112 | 129 | 1.6 | 0.08 | 0.64 | 0.02 |
| 99.99 | 591 657 | 203 | 2.9 | 0.11 | 0.64 | 0.023 |

Table 104: AMUB-FRML, 2 qubits, random noisy preparation

| $F_B, \%$ | $N_B$ | $M_B$ | $T_{P,B}$, sec | $T_{E,B}$, sec | $\eta_B$ | $O_B$ |
|---|---|---|---|---|---|---|
| 90 | *91 | – | – | – | – | – |
| 99 | 15 089 | 83 | 2.5 | 0.27 | 0.27 | 0.021 |
| 99.9 | 165 667 | 161 | 5.2 | 0.2 | 0.28 | 0.0083 |
| 99.99 | 2 641 111 | 252 | 9.6 | 0.36 | 0.19 | 0.019 |

### 9.3 3 qubits

Table 105: AMUB-FRML, 3 qubits, random pure states

| $F_B, \%$ | $N_B$ | $M_B$ | $T_{P,B}$, sec | $T_{E,B}$, sec | $\eta_B$ | $O_B$ |
|---|---|---|---|---|---|---|
| 90 | 836 | 17 | 0.44 | 0.8 | 0.14 | 0.0097 |
| 99 | 5 976 | 60 | 9.7 | 2.7 | 0.24 | 0.0038 |
| 99.9 | 48 859 | 128 | 44 | 11 | 0.31 | 0.002 |
| 99.99 | 431 966 | 204 | 142 | 17 | 0.37 | 0.0014 |

Table 106: AMUB-FRML, 3 qubits, random mixed states by partial tracing (rank-2) test

| $F_B, \%$ | $N_B$ | $M_B$ | $T_{P,B}$, sec | $T_{E,B}$, sec | $\eta_B$ | $O_B$ |
|---|---|---|---|---|---|---|
| 90 | 1 319 | 24 | 2.4 | 1.4 | 0.31 | 0.016 |
| 99 | 15 375 | 87 | 37 | 12 | 0.32 | 0.015 |
| 99.9 | 141 855 | 165 | 180 | 35 | 0.33 | 0.012 |
| 99.99 | 1 466 307 | 247 | 555 | 67 | 0.32 | 0.0092 |

Table 107: AMUB-FRML, 3 qubits, random mixed states by partial tracing (full-rank) test

| $F_B, \%$ | $N_B$ | $M_B$ | $T_{P,B}$, sec | $T_{E,B}$, sec | $\eta_B$ | $O_B$ |
|---|---|---|---|---|---|---|
| 90 | *201 | – | – | – | – | – |
| 99 | 40 412 | 121 | 33 | 5.3 | 0.55 | 0.02 |
| 99.9 | 439 161 | 205 | 106 | 11 | 0.52 | 0.022 |
| 99.99 | 5 063 846 | 291 | 234 | 17 | 0.48 | 0.025 |

Table 108: AMUB-FRML, 3 qubits, random noisy preparation

| $F_B, \%$ | $N_B$ | $M_B$ | $T_{P,B}$, sec | $T_{E,B}$, sec | $\eta_B$ | $O_B$ |
|---|---|---|---|---|---|---|
| 90 | *263 | – | – | – | – | – |
| 99 | 74 506 | 143 | 256 | 68 | 0.28 | 0.019 |
| 99.9 | 1 317 030 | 244 | 1 067 | 66 | 0.19 | 0.009 |
| 99.99 | *11 965 326 | – | – | – | – | – |

## 10 FO-FRML

- Protocol: factorized orthogonal [3]

- Estimator: full-rank maximum likelihood
- Algorithm: full-rank root approach estimator using [8]
- Machine: Intel(R) Xeon(R) CPU E5450 @ 3.00GHz

### 10.1 2 qubits

Table 109: FO-FRML, 2 qubits, random pure states

| $F_B$, % | $N_B$ | $M_B$ | $T_{P,B}$, sec | $T_{E,B}$, sec | $\eta_B$ | $O_B$ |
|---|---|---|---|---|---|---|
| 90 | 789 | 9 | 141 | 0.16 | 0.098 | 0.015 |
| 99 | 8 167 | 62 | 161 | 0.13 | 0.11 | 0.027 |
| 99.9 | 164 734 | 153 | 170 | 0.14 | 0.062 | 0.048 |
| 99.99 | *1 094 231 | – | – | – | – | – |

Table 110: FO-FRML, 2 qubits, random mixed states by partial tracing (rank-2) test

| $F_B$, % | $N_B$ | $M_B$ | $T_{P,B}$, sec | $T_{E,B}$, sec | $\eta_B$ | $O_B$ |
|---|---|---|---|---|---|---|
| 90 | 2 275 | 30 | 97 | 0.35 | 0.16 | 0.032 |
| 99 | 17 834 | 85 | 110 | 0.52 | 0.17 | 0.01 |
| 99.9 | 353 999 | 176 | 166 | 1.4 | 0.097 | 0.05 |
| 99.99 | *1 277 361 | – | – | – | – | – |

Table 111: FO-FRML, 2 qubits, random mixed states by partial tracing (full-rank) test

| $F_B$, % | $N_B$ | $M_B$ | $T_{P,B}$, sec | $T_{E,B}$, sec | $\eta_B$ | $O_B$ |
|---|---|---|---|---|---|---|
| 90 | 3 323 | 40 | 108 | 0.78 | 0.15 | 0.028 |
| 99 | 65 133 | 125 | 152 | 0.76 | 0.087 | 0.026 |
| 99.9 | 3 446 412 | 246 | 328 | 4.1 | 0.02 | 0.016 |
| 99.99 | *17 364 377 | – | – | – | – | – |

Table 112: FO-FRML, 2 qubits, random noisy preparation

| $F_B$, % | $N_B$ | $M_B$ | $T_{P,B}$, sec | $T_{E,B}$, sec | $\eta_B$ | $O_B$ |
|---|---|---|---|---|---|---|
| 90 | 1 263 | 16 | 130 | 0.27 | 0.3 | 0.019 |
| 99 | 47 114 | 115 | 164 | 0.65 | 0.11 | 0.013 |
| 99.9 | 2 851 554 | 240 | 301 | 3.5 | 0.026 | 0.014 |
| 99.99 | *18 236 562 | – | – | – | – | – |

### 10.2 3 qubits

Table 113: FO-FRML, 3 qubits, random pure states

| $F_B$, % | $N_B$ | $M_B$ | $T_{P,B}$, sec | $T_{E,B}$, sec | $\eta_B$ | $O_B$ |
|---:|---:|---:|---:|---:|---:|---:|
| 90 | 1 448 | 19 | 220 | 1.4 | 0.099 | 0.013 |
| 99 | 12 103 | 73 | 275 | 3.8 | 0.12 | 0.0076 |
| 99.9 | 139 756 | 148 | 563 | 4.1 | 0.12 | 0.013 |
| 99.99 | *1 057 832 | – | – | – | – | – |

Table 114: FO-FRML, 3 qubits, random mixed states by partial tracing (rank-2) test

| $F_B$, % | $N_B$ | $M_B$ | $T_{P,B}$, sec | $T_{E,B}$, sec | $\eta_B$ | $O_B$ |
|---:|---:|---:|---:|---:|---:|---:|
| 90 | 2 922 | 37 | 268 | 3.3 | 0.17 | 0.02 |
| 99 | 30 208 | 101 | 522 | 8 | 0.16 | 0.014 |
| 99.9 | 337 222 | 175 | 1 417 | 18 | 0.15 | 0.014 |
| 99.99 | 3 570 553 | 247 | 2 965 | 31 | 0.14 | 0.012 |

Table 115: FO-FRML, 3 qubits, random mixed states by partial tracing (full-rank) test

| $F_B$, % | $N_B$ | $M_B$ | $T_{P,B}$, sec | $T_{E,B}$, sec | $\eta_B$ | $O_B$ |
|---:|---:|---:|---:|---:|---:|---:|
| 90 | *6 255 | – | – | – | – | – |
| 99 | 306 509 | 172 | 3 809 | 68 | 0.09 | 0.016 |
| 99.9 | 9 496 329 | 276 | 15 619 | 204 | 0.045 | 0.054 |
| 99.99 | *16 953 520 | – | – | – | – | – |

Table 116: FO-FRML, 3 qubits, random noisy preparation

| $F_B$, % | $N_B$ | $M_B$ | $T_{P,B}$, sec | $T_{E,B}$, sec | $\eta_B$ | $O_B$ |
|---:|---:|---:|---:|---:|---:|---:|
| 90 | *990 | – | – | – | – | – |
| 99 | 196 801 | 159 | 2 772 | 55 | 0.11 | 0.015 |
| 99.9 | *13 688 307 | – | – | – | – | – |
| 99.99 | *26 032 648 | – | – | – | – | – |

## 11 FOMUB-FRML

- Protocol: factorized orthogonal mutually unbiased bases [4]
- Estimator: full-rank maximum likelihood
- Algorithm: full-rank root approach estimator using [8]
- Machine: Intel(R) Xeon(R) CPU E5450 @ 3.00GHz

### 11.1 2 qubits

Table 117: FOMUB-FRML, 2 qubits, random pure states

| $F_B$,% | $N_B$ | $M_B$ | $T_{P,B}$, sec | $T_{E,B}$, sec | $\eta_B$ | $O_B$ |
|---|---|---|---|---|---|---|
| 90 | 300 | 13 | 0.17 | 0.22 | 0.23 | 0.002 |
| 99 | 9 398 | 71 | 4.6 | 0.91 | 0.092 | 0.002 |
| 99.9 | 172 765 | 172 | 15 | 1.1 | 0.073 | 0.0078 |
| 99.99 | *1 130 390 | – | – | – | – | – |

Table 118: FOMUB-FRML, 2 qubits, random mixed states by partial tracing (rank-2) test

| $F_B$,% | $N_B$ | $M_B$ | $T_{P,B}$, sec | $T_{E,B}$, sec | $\eta_B$ | $O_B$ |
|---|---|---|---|---|---|---|
| 90 | 491 | 15 | 0.27 | 0.32 | 0.48 | 0.012 |
| 99 | 13 475 | 82 | 7.1 | 1.3 | 0.22 | 0.001 |
| 99.9 | 217 640 | 180 | 20 | 2 | 0.16 | 0.013 |
| 99.99 | *1 205 477 | – | – | – | – | – |

Table 119: FOMUB-FRML, 2 qubits, random mixed states by partial tracing (full-rank) test

| $F_B$,% | $N_B$ | $M_B$ | $T_{P,B}$, sec | $T_{E,B}$, sec | $\eta_B$ | $O_B$ |
|---|---|---|---|---|---|---|
| 90 | *704 | – | – | – | – | – |
| 99 | 15 580 | 88 | 7.7 | 0.72 | 0.33 | 0.048 |
| 99.9 | 268 040 | 188 | 20 | 0.84 | 0.24 | 0.073 |
| 99.99 | 4 249 725 | 285 | 33 | 1.1 | 0.1 | 0.098 |

Table 120: FOMUB-FRML, 2 qubits, random noisy preparation

| $F_B$,% | $N_B$ | $M_B$ | $T_{P,B}$, sec | $T_{E,B}$, sec | $\eta_B$ | $O_B$ |
|---|---|---|---|---|---|---|
| 90 | *265 | – | – | – | – | – |
| 99 | 24 257 | 103 | 8.9 | 1.5 | 0.17 | 0.022 |
| 99.9 | 629 755 | 218 | 36 | 2.1 | 0.095 | 0.036 |
| 99.99 | 5 763 044 | 296 | 54 | 1.9 | 0.093 | 0.038 |

### 11.2 3 qubits

Table 121: FOMUB-FRML, 3 qubits, random pure states

| $F_B$,% | $N_B$ | $M_B$ | $T_{P,B}$, sec | $T_{E,B}$, sec | $\eta_B$ | $O_B$ |
|---|---|---|---|---|---|---|
| 90 | 715 | 27 | 0.014 | 1.7 | 0.17 | 0.009 |
| 99 | 34 224 | 139 | 155 | 96 | 0.035 | 0.0068 |
| 99.9 | *1 301 485 | – | – | – | – | – |
| 99.99 | *2 251 263 | – | – | – | – | – |

Table 122: FOMUB-FRML, 3 qubits, random mixed states by partial tracing (rank-2) test

| $F_B, \%$ | $N_B$ | $M_B$ | $T_{P,B}$, sec | $T_{E,B}$, sec | $\eta_B$ | $O_B$ |
|---|---|---|---|---|---|---|
| 90 | 1 873 | 42 | 4 | 7.3 | 0.22 | 0.011 |
| 99 | 107 701 | 192 | 506 | 385 | 0.04 | 0.0042 |
| 99.9 | 7 270 918 | 367 | 9 828 | 4 927 | 0.0068 | 0.0066 |
| 99.99 | *21 890 735 | – | – | – | – | – |

Table 123: FOMUB-FRML, 3 qubits, random mixed states by partial tracing (full-rank) test

| $F_B, \%$ | $N_B$ | $M_B$ | $T_{P,B}$, sec | $T_{E,B}$, sec | $\eta_B$ | $O_B$ |
|---|---|---|---|---|---|---|
| 90 | *1 148 | – | – | – | – | – |
| 99 | 124 270 | 199 | 288 | 165 | 0.2 | 0.0095 |
| 99.9 | 9 671 663 | 377 | 2 588 | 692 | 0.063 | 0.093 |
| 99.99 | *34 353 230 | – | – | – | – | – |

Table 124: FOMUB-FRML, 3 qubits, random noisy preparation

| $F_B, \%$ | $N_B$ | $M_B$ | $T_{P,B}$, sec | $T_{E,B}$, sec | $\eta_B$ | $O_B$ |
|---|---|---|---|---|---|---|
| 90 | *452 | – | – | – | – | – |
| 99 | 164 533 | 212 | 626 | 488 | 0.12 | 0.018 |
| 99.9 | *14 320 719 | – | – | – | – | – |
| 99.99 | *29 807 799 | – | – | – | – | – |

# 12 SGQT

- Method: Self-guided quantum tomography [5]
- Machine: Intel(R) Xeon(R) CPU E5450 @ 3.00GHz

## 12.1 1 qubit

Table 125: SGQT, 1 qubit, random pure states

| $F_B, \%$ | $N_B$ | $M_B$ | $T_{P,B}$, sec | $T_{E,B}$, sec | $\eta_B$ | $O_B$ |
|---|---|---|---|---|---|---|
| 90 | 27 157 | 490 | 0.092 | 0.00016 | 0.0014 | 0.0039 |
| 99 | 87 626 | 948 | 0.18 | 0.00018 | 0.0042 | 0.0085 |
| 99.9 | *1 019 437 | – | – | – | – | – |
| 99.99 | *1 391 690 | – | – | – | – | – |

### 12.2 2 qubits

Table 126: SGQT, 2 qubits, random pure states

| $F_B, \%$ | $N_B$ | $M_B$ | $T_{P,B}$, sec | $T_{E,B}$, sec | $\eta_B$ | $O_B$ |
|---|---|---|---|---|---|---|
| 90 | 175 432 | 3 197 | 0.5 | 0.00019 | 0.00044 | 0.0032 |
| 99 | 730 382 | 8 772 | 1.4 | 0.00023 | 0.00096 | 0.0088 |
| 99.9 | *1 048 989 | – | – | – | – | – |
| 99.99 | *1 058 019 | – | – | – | – | – |

### 12.3 3 qubits

Table 127: SGQT, 3 qubits, random pure states

| $F_B, \%$ | $N_B$ | $M_B$ | $T_{P,B}$, sec | $T_{E,B}$, sec | $\eta_B$ | $O_B$ |
|---|---|---|---|---|---|---|
| 90 | 505 422 | 7 333 | 1.1 | 0.00017 | 0.00024 | 0.0057 |
| 99 | *1 134 104 | – | – | – | – | – |
| 99.9 | *1 171 792 | – | – | – | – | – |
| 99.99 | *1 175 629 | – | – | – | – | – |

## References


[1] Steffens A. et al. Experimentally exploring compressed sensing quantum tomography // Quantum Sci. Technol. 2017. Vol. 2, 2. P. 025005.

[2] Flammia S.T. et al. Quantum tomography via compressed sensing: error bounds, sample complexity and efficient estimators // New J. Phys. 2012. Vol. 14, 9. P. 095022.

[3] Struchalin G.I. et al. Adaptive quantum tomography of high-dimensional bipartite systems // Phys. Rev. A. American Physical Society, 2018. Vol. 98, 3. P. 032330.

[4] JETP TODO.

[5] Ferrie C. Self-Guided Quantum Tomography // Phys. Rev. Lett. American Physical Society, 2014. Vol. 113, 19. P. 190404.

[6] Efficient MATLAB routines for quantum tomography [Electronic resource]. URL: https://github.com/qMLE/qMLE.

[7] Grant M., Boyd S. CVX: Matlab software for disciplined convex programming, version 2.0 beta [Electronic resource]. 2013. URL: http://cvxr.com/cvx.

[8] Quantum tomography by MLE and root approach [Electronic resource]. URL: https://github.com/PQCLab/RootTomography.
