# Supplementary material for: Quantum tomography benchmarking
Source: arXiv:2012.15656 source file (2021-10-11)
Supplement: Supplementary file 2 [file Supplementary2.pdf]

# Supplementary material II. Methods comparison

Quantum tomography benchmarking
Bantysh B. I., Chernyavskiy A. Yu., Bogdanov Yu. I.

The current document summarizes the relative performance of various quantum tomography methods using the results presented in Supplementary material I. The sign "*" in tables means that the value was obtained by linear extrapolation of the dependence of $\log[1-F]_{95}$ on $\log N$.

## Contents

**1 Random pure states test** **2**
- 1.1 1 qubit . . . 2
- 1.2 2 qubits . . . 4
- 1.3 3 qubits . . . 6

**2 Random mixed states by partial tracing (rank-2) test** **8**
- 2.1 1 qubit . . . 8
- 2.2 2 qubits . . . 10
- 2.3 3 qubits . . . 12

**3 Random mixed states by partial tracing (full-rank) test** **14**
- 3.1 1 qubit . . . 14
- 3.2 2 qubits . . . 16
- 3.3 3 qubits . . . 18

**4 Random noisy preparation test** **20**
- 4.1 1 qubit . . . 20
- 4.2 2 qubits . . . 22
- 4.3 3 qubits . . . 24

# 1 Random pure states test

## 1.1 1 qubit

Table 1: Random pure states test, 1 qubit, $F_B = 90\%$

| | $N_B$ | $M_B$ | $T_{P,B}$, sec | $T_{E,B}$, sec | $\eta_B$ | $O_B$ |
|---|---|---|---|---|---|---|
| **Lower bound** | 30 | – | – | – | 1 | – |
| **MUB–ARML** | *1 | – | – | – | – | – |
| **AMUB–ARML** | *1 | – | – | – | – | – |
| **FMUB–ARML** | *1 | – | – | – | – | – |
| **FMUB–TRML** | *1 | – | – | – | – | – |
| **PAULI–CS** | *1 | – | – | – | – | – |
| **FMUB–CS** | *2 | – | – | – | – | – |
| **MUB–FRML** | *83 | – | – | – | – | – |
| **FMUB–FRML** | *83 | – | – | – | – | – |
| **FMUB–FRLS** | *83 | – | – | – | – | – |
| **FMUB–PPI** | *83 | – | – | – | – | – |
| **AMUB–FRML** | *86 | – | – | – | – | – |
| **SGQT** | 27 157 | 490 | 0.092 | 0.00016 | 0.0014 | 0.0039 |

Table 2: Random pure states test, 1 qubit, $F_B = 99\%$

| | $N_B$ | $M_B$ | $T_{P,B}$, sec | $T_{E,B}$, sec | $\eta_B$ | $O_B$ |
|---|---|---|---|---|---|---|
| **Lower bound** | 300 | – | – | – | 1 | – |
| **FMUB–TRML** | 339 | 3 | 0.00052 | 0.0058 | 0.91 | 0.0064 |
| **PAULI–CS** | 344 | 3 | 0.00037 | 0.66 | 0.84 | 0.0049 |
| **MUB–ARML** | 381 | 3 | 0.00049 | 0.0063 | 0.63 | 0.02 |
| **FMUB–ARML** | 381 | 3 | 0.00069 | 0.009 | 0.63 | 0.02 |
| **AMUB–ARML** | 570 | 10 | 1 | 0.018 | 0.65 | 0.02 |
| **FMUB–CS** | 599 | 3 | 0.00034 | 0.47 | 0.56 | 0.023 |
| **AMUB–FRML** | 990 | 12 | 0.067 | 0.027 | 0.41 | 0.032 |
| **MUB–FRML** | 9 881 | 3 | 0.00053 | 0.0055 | 0.045 | 0 |
| **FMUB–FRML** | 9 881 | 3 | 0.00041 | 0.0037 | 0.045 | 0 |
| **FMUB–FRLS** | 9 881 | 3 | 0.00045 | 0.54 | 0.045 | 0 |
| **FMUB–PPI** | 9 881 | 3 | 0.00035 | 0.0006 | 0.045 | 0 |
| **SGQT** | 87 626 | 948 | 0.18 | 0.00018 | 0.0042 | 0.0085 |

Table 3: Random pure states test, 1 qubit, $F_B = 99.9\%$

| | $N_B$ | $M_B$ | $T_{P,B}$, sec | $T_{E,B}$, sec | $\eta_B$ | $O_B$ |
|---|---|---|---|---|---|---|
| **Lower bound** | 2 996 | – | – | – | 1 | – |
| **PAULI–CS** | 3 379 | 3 | 0.00038 | 0.66 | 0.85 | 0.0051 |
| **FMUB–TRML** | 3 387 | 3 | 0.00053 | 0.0059 | 0.9 | 0.004 |
| **MUB–ARML** | 4 429 | 3 | 0.00046 | 0.0063 | 0.28 | 0.027 |
| **FMUB–ARML** | 4 429 | 3 | 0.00071 | 0.0088 | 0.28 | 0.027 |
| **AMUB–ARML** | 7 127 | 61 | 1 | 0.031 | 0.56 | 0.037 |
| **AMUB–FRML** | 8 802 | 66 | 0.73 | 0.04 | 0.46 | 0.015 |
| **FMUB–CS** | 56 212 | 3 | 0.00034 | 0.44 | 0.11 | 0.11 |
| **FMUB–FRLS** | 867 380 | 3 | 0.00042 | 0.55 | 0.005 | 0 |
| **FMUB–PPI** | 867 383 | 3 | 0.00035 | 0.00055 | 0.005 | 0 |
| **MUB–FRML** | 867 389 | 3 | 0.00049 | 0.0052 | 0.005 | 0 |
| **FMUB–FRML** | 867 389 | 3 | 0.00036 | 0.0036 | 0.005 | 0 |
| **SGQT** | *1 019 437 | – | – | – | – | – |

Table 4: Random pure states test, 1 qubit, $F_B = 99.99\%$

| | $N_B$ | $M_B$ | $T_{P,B}$, sec | $T_{E,B}$, sec | $\eta_B$ | $O_B$ |
|---|---|---|---|---|---|---|
| **Lower bound** | 29 957 | – | – | – | 1 | – |
| **FMUB–TRML** | 32 859 | 3 | 0.00055 | 0.0055 | 0.92 | 0.0061 |
| **PAULI–CS** | 35 069 | 3 | 0.00038 | 0.68 | 0.85 | 0.0033 |
| **MUB–ARML** | 43 310 | 3 | 0.00045 | 0.0062 | 0.12 | 0.029 |
| **FMUB–ARML** | 43 310 | 3 | 0.00065 | 0.0088 | 0.12 | 0.029 |
| **AMUB–ARML** | 91 836 | 138 | 1.3 | 0.045 | 0.48 | 0.028 |
| **AMUB–FRML** | 106 287 | 143 | 1.6 | 0.04 | 0.35 | 0.0051 |
| **SGQT** | *1 391 690 | – | – | – | – | – |
| **FMUB–CS** | *1 811 808 | – | – | – | – | – |
| **FMUB–FRLS** | *2 589 217 | – | – | – | – | – |
| **FMUB–PPI** | *2 589 225 | – | – | – | – | – |
| **MUB–FRML** | *2 589 235 | – | – | – | – | – |
| **FMUB–FRML** | *2 589 235 | – | – | – | – | – |

### 1.2 2 qubits

Table 5: Random pure states test, 2 qubits, $F_B = 90\%$

| | $N_B$ | $M_B$ | $T_{P,B}$, sec | $T_{E,B}$, sec | $\eta_B$ | $O_B$ | FM |
|---|---|---|---|---|---|---|---|
| **Lower bound** | 63 | – | – | – | 1 | – | – |
| **FMUB–TRML** | *63 | – | – | – | – | – | Y |
| **MUB–ARML** | *83 | – | – | – | – | – | N |
| **AMUB–ARML** | *83 | – | – | – | – | – | N |
| **FOMUB–ARML** | *88 | – | – | – | – | – | Y |
| **FMUB–ARML** | *89 | – | – | – | – | – | Y |
| **FMUB–CS** | 220 | 9 | 0.0008 | 1 | 0.37 | 0.029 | Y |
| **AMUB–FRML** | 228 | 7 | 0.04 | 0.12 | 0.32 | 0.0026 | N |
| **FOMUB–FRML** | 300 | 13 | 0.17 | 0.22 | 0.23 | 0.002 | Y |
| **FMUB–FRML** | 321 | 9 | 0.00094 | 0.034 | 0.22 | 0.0025 | Y |
| **PAULI–CS** | 341 | 15 | 0.0018 | 0.79 | 0.14 | 0.0055 | Y |
| **MUB–FRML** | 381 | 5 | 0.00057 | 0.029 | 0.18 | 0.0017 | N |
| **FO–ARML** | 400 | 6 | 53 | 0.031 | 0.16 | 0.044 | Y |
| **FMUB–FRLS** | 519 | 9 | 0.00092 | 0.47 | 0.13 | 0 | Y |
| **FMUB–PPI** | 568 | 9 | 0.00064 | 0.00055 | 0.12 | 0.0015 | Y |
| **FO–FRML** | 789 | 9 | 141 | 0.16 | 0.098 | 0.015 | Y |
| **SGQT** | 175 432 | 3 197 | 0.5 | 0.00019 | 0.00044 | 0.0032 | N |

Table 6: Random pure states test, 2 qubits, $F_B = 99\%$

| | $N_B$ | $M_B$ | $T_{P,B}$, sec | $T_{E,B}$, sec | $\eta_B$ | $O_B$ | FM |
|---|---|---|---|---|---|---|---|
| **Lower bound** | 630 | – | – | – | 1 | – | – |
| **FMUB–TRML** | 750 | 9 | 0.0013 | 0.0079 | 0.89 | 0.024 | Y |
| **MUB–ARML** | 782 | 5 | 0.00057 | 0.0063 | 0.7 | 0.02 | N |
| **FMUB–ARML** | 801 | 9 | 0.0014 | 0.013 | 0.68 | 0.054 | Y |
| **AMUB–ARML** | 844 | 10 | 0.013 | 0.026 | 0.74 | 0.036 | N |
| **FOMUB–ARML** | 1 476 | 27 | 0.19 | 0.055 | 0.56 | 0.058 | Y |
| **PAULI–CS** | 2 034 | 15 | 0.0019 | 0.8 | 0.31 | 0.0066 | Y |
| **AMUB–FRML** | 2 632 | 35 | 0.87 | 0.21 | 0.31 | 0.0013 | N |
| **FO–ARML** | 3 050 | 38 | 91 | 0.064 | 0.32 | 0.079 | Y |
| **FO–FRML** | 8 167 | 62 | 161 | 0.13 | 0.11 | 0.027 | Y |
| **FOMUB–FRML** | 9 398 | 71 | 4.6 | 0.91 | 0.092 | 0.002 | Y |
| **FMUB–CS** | 13 959 | 9 | 0.00084 | 0.76 | 0.092 | 0.037 | Y |
| **FMUB–FRML** | 23 990 | 9 | 0.00094 | 0.15 | 0.029 | 0.0035 | Y |
| **MUB–FRML** | 33 864 | 5 | 0.00061 | 0.16 | 0.02 | 0.0029 | N |
| **FMUB–FRLS** | 46 413 | 9 | 0.00094 | 0.48 | 0.014 | 0.0027 | Y |
| **FMUB–PPI** | 50 976 | 9 | 0.00063 | 0.00056 | 0.013 | 0.0027 | Y |
| **SGQT** | 730 382 | 8 772 | 1.4 | 0.00023 | 0.00096 | 0.0088 | N |

Table 7: Random pure states test, 2 qubits, $F_B = 99.9\%$

| | $N_B$ | $M_B$ | $T_{P,B}$, sec | $T_{E,B}$, sec | $\eta_B$ | $O_B$ | FM |
|---:|---:|---:|---:|---:|---:|---:|---:|
| **Lower bound** | 6 296 | – | – | – | 1 | – | – |
| **FMUB–TRML** | 7 205 | 9 | 0.0014 | 0.0081 | 0.9 | 0.0098 | Y |
| **MUB–ARML** | 7 559 | 5 | 0.00057 | 0.0063 | 0.56 | 0.023 | N |
| **FMUB–ARML** | 7 798 | 9 | 0.0014 | 0.013 | 0.57 | 0.022 | Y |
| **FOMUB–ARML** | 13 402 | 82 | 0.86 | 0.11 | 0.49 | 0.052 | Y |
| **AMUB–ARML** | 19 082 | 91 | 1.1 | 0.097 | 0.6 | 0.083 | N |
| **PAULI–CS** | 20 239 | 15 | 0.0019 | 0.84 | 0.31 | 0.0071 | Y |
| **AMUB–FRML** | 23 472 | 98 | 2.9 | 0.31 | 0.35 | 0.0026 | N |
| **FO–ARML** | 39 134 | 109 | 97 | 0.086 | 0.29 | 0.076 | Y |
| **FO–FRML** | 164 734 | 153 | 170 | 0.14 | 0.062 | 0.048 | Y |
| **FOMUB–FRML** | 172 765 | 172 | 15 | 1.1 | 0.073 | 0.0078 | Y |
| **SGQT** | *1 048 989 | – | – | – | – | – | N |
| **FMUB–CS** | *1 123 593 | – | – | – | – | – | Y |
| **FMUB–FRML** | *1 424 621 | – | – | – | – | – | Y |
| **MUB–FRML** | *1 638 550 | – | – | – | – | – | N |
| **FMUB–FRLS** | *1 763 979 | – | – | – | – | – | Y |
| **FMUB–PPI** | *1 811 355 | – | – | – | – | – | Y |

Table 8: Random pure states test, 2 qubits, $F_B = 99.99\%$

| | $N_B$ | $M_B$ | $T_{P,B}$, sec | $T_{E,B}$, sec | $\eta_B$ | $O_B$ | FM |
|---:|---:|---:|---:|---:|---:|---:|---:|
| **Lower bound** | 62 958 | – | – | – | 1 | – | – |
| **FMUB–TRML** | 70 588 | 9 | 0.0013 | 0.0077 | 0.92 | 0.0045 | Y |
| **MUB–ARML** | 73 128 | 5 | 0.00057 | 0.0078 | 0.29 | 0.022 | N |
| **FMUB–ARML** | 75 357 | 9 | 0.0014 | 0.011 | 0.36 | 0.014 | Y |
| **AMUB–ARML** | 171 291 | 163 | 2.8 | 0.14 | 0.61 | 0.058 | N |
| **PAULI–CS** | 206 950 | 15 | 0.0019 | 0.86 | 0.31 | 0.005 | Y |
| **AMUB–FRML** | 229 502 | 172 | 6.2 | 0.33 | 0.37 | 0.015 | N |
| **FOMUB–ARML** | 322 224 | 194 | 3.3 | 0.24 | 0.35 | 0.076 | Y |
| **FO–ARML** | 410 514 | 181 | 108 | 0.12 | 0.27 | 0.097 | Y |
| **SGQT** | *1 058 019 | – | – | – | – | – | N |
| **FO–FRML** | *1 094 231 | – | – | – | – | – | Y |
| **FOMUB–FRML** | *1 130 390 | – | – | – | – | – | Y |
| **FMUB–FRML** | *2 655 567 | – | – | – | – | – | Y |
| **FMUB–CS** | *2 710 677 | – | – | – | – | – | Y |
| **FMUB–FRLS** | *2 742 326 | – | – | – | – | – | Y |
| **MUB–FRML** | *2 748 077 | – | – | – | – | – | N |
| **FMUB–PPI** | *2 770 068 | – | – | – | – | – | Y |

### 1.3 3 qubits

Table 9: Random pure states test, 3 qubits, $F_B = 90\%$

| | $N_B$ | $M_B$ | $T_{P,B}$, sec | $T_{E,B}$, sec | $\eta_B$ | $O_B$ | FM |
|---:|---:|---:|---:|---:|---:|---:|:---:|
| **Lower bound** | 118 | – | – | – | 1 | – | – |
| **MUB–ARML** | 158 | 9 | 0.0011 | 0.015 | 0.81 | 0.034 | N |
| **FMUB–TRML** | 163 | 27 | 0.002 | 0.014 | 0.81 | 0.019 | Y |
| **FMUB–ARML** | 167 | 27 | 0.0018 | 0.015 | 0.77 | 0.027 | Y |
| **FOMUB–ARML** | 186 | 27 | 0.016 | 0.11 | 0.72 | 0.023 | Y |
| **AMUB–ARML** | 256 | 13 | 0.017 | 0.1 | 0.73 | 0.074 | N |
| **FO–ARML** | 669 | 8 | 0.88 | 0.17 | 0.31 | 0.095 | Y |
| **FMUB–FRML** | 713 | 27 | 0.0021 | 0.25 | 0.17 | 0.0083 | Y |
| **FOMUB–FRML** | 715 | 27 | 0.014 | 1.7 | 0.17 | 0.009 | Y |
| **FMUB–CS** | 751 | 27 | 0.0018 | 0.87 | 0.22 | 0.0028 | Y |
| **AMUB–FRML** | 836 | 17 | 0.44 | 0.8 | 0.14 | 0.0097 | N |
| **MUB–FRML** | 903 | 9 | 0.00054 | 0.076 | 0.13 | 0.0022 | N |
| **FO–FRML** | 1 448 | 19 | 220 | 1.4 | 0.099 | 0.013 | Y |
| **FMUB–FRLS** | 1 574 | 27 | 0.002 | 0.53 | 0.073 | 0.0048 | Y |
| **FMUB–PPI** | 2 134 | 27 | 0.0025 | 0.0034 | 0.053 | 0.0077 | Y |
| **PAULI–CS** | 2 245 | 63 | 0.0079 | 1.1 | 0.089 | 0.071 | Y |
| **SGQT** | 505 422 | 7 333 | 1.1 | 0.00017 | 0.00024 | 0.0057 | N |

Table 10: Random pure states test, 3 qubits, $F_B = 99\%$

| | $N_B$ | $M_B$ | $T_{P,B}$, sec | $T_{E,B}$, sec | $\eta_B$ | $O_B$ | FM |
|---:|---:|---:|---:|---:|---:|---:|:---:|
| **Lower bound** | 1 184 | – | – | – | 1 | – | – |
| **FMUB–TRML** | 1 380 | 27 | 0.002 | 0.011 | 0.89 | 0.0081 | Y |
| **MUB–ARML** | 1 468 | 9 | 0.0011 | 0.018 | 0.71 | 0.029 | N |
| **FMUB–ARML** | 1 565 | 27 | 0.0019 | 0.016 | 0.68 | 0.036 | Y |
| **AMUB–ARML** | 4 210 | 52 | 1.4 | 0.48 | 0.64 | 0.11 | N |
| **FOMUB–ARML** | 4 887 | 64 | 0.84 | 0.52 | 0.54 | 0.064 | Y |
| **AMUB–FRML** | 5 976 | 60 | 9.7 | 2.7 | 0.24 | 0.0038 | N |
| **FO–ARML** | 6 133 | 55 | 1 | 0.55 | 0.47 | 0.11 | Y |
| **PAULI–CS** | 9 087 | 63 | 0.0081 | 1.1 | 0.14 | 0.018 | Y |
| **FO–FRML** | 12 103 | 73 | 275 | 3.8 | 0.12 | 0.0076 | Y |
| **FOMUB–FRML** | 34 224 | 139 | 155 | 96 | 0.035 | 0.0068 | Y |
| **FMUB–CS** | 47 889 | 27 | 0.0019 | 0.77 | 0.046 | 0.00068 | Y |
| **FMUB–FRML** | 48 133 | 27 | 0.0022 | 1.1 | 0.025 | 0.0054 | Y |
| **MUB–FRML** | 83 906 | 9 | 0.00055 | 0.55 | 0.014 | 0.0038 | N |
| **FMUB–FRLS** | 150 722 | 27 | 0.0021 | 0.54 | 0.0077 | 0.0075 | Y |
| **FMUB–PPI** | 203 021 | 27 | 0.0025 | 0.0036 | 0.0056 | 0.019 | Y |
| **SGQT** | *1 134 104 | – | – | – | – | – | N |

Table 11: Random pure states test, 3 qubits, $F_B = 99.9\%$

| | $N_B$ | $M_B$ | $T_{P,B}$, sec | $T_{E,B}$, sec | $\eta_B$ | $O_B$ | FM |
|---:|---:|---:|---:|---:|---:|---:|---:|
| **Lower bound** | 11 842 | – | – | – | 1 | – | – |
| **FMUB–TRML** | 12 960 | 27 | 0.0021 | 0.011 | 0.92 | 0.015 | Y |
| **MUB–ARML** | 14 148 | 9 | 0.0011 | 0.035 | 0.48 | 0.039 | N |
| **FMUB–ARML** | 15 381 | 27 | 0.0018 | 0.037 | 0.5 | 0.039 | Y |
| **FOMUB–ARML** | 35 286 | 140 | 5.8 | 0.99 | 0.37 | 0.066 | Y |
| **AMUB–ARML** | 37 419 | 118 | 10 | 2.1 | 0.66 | 0.1 | N |
| **AMUB–FRML** | 48 859 | 128 | 44 | 11 | 0.31 | 0.002 | N |
| **FO–ARML** | 75 905 | 129 | 1 | 1.3 | 0.41 | 0.16 | Y |
| **PAULI–CS** | 83 740 | 63 | 0.008 | 1.1 | 0.14 | 0.0085 | Y |
| **FO–FRML** | 139 756 | 148 | 563 | 4.1 | 0.12 | 0.013 | Y |
| **SGQT** | *1 171 792 | – | – | – | – | – | N |
| **FOMUB–FRML** | *1 301 485 | – | – | – | – | – | Y |
| **FMUB–FRML** | *1 791 982 | – | – | – | – | – | Y |
| **MUB–FRML** | *2 007 764 | – | – | – | – | – | N |
| **FMUB–FRLS** | *2 178 934 | – | – | – | – | – | Y |
| **FMUB–CS** | *2 187 271 | – | – | – | – | – | Y |
| **FMUB–PPI** | *2 300 913 | – | – | – | – | – | Y |

Table 12: Random pure states test, 3 qubits, $F_B = 99.99\%$

| | $N_B$ | $M_B$ | $T_{P,B}$, sec | $T_{E,B}$, sec | $\eta_B$ | $O_B$ | FM |
|---:|---:|---:|---:|---:|---:|---:|---:|
| **Lower bound** | 118 424 | – | – | – | 1 | – | – |
| **MUB–ARML** | 130 039 | 9 | 0.0011 | 0.018 | 0.4 | 0.013 | N |
| **FMUB–TRML** | 133 258 | 27 | 0.0021 | 0.01 | 0.93 | 0.011 | Y |
| **FMUB–ARML** | 143 532 | 27 | 0.0019 | 0.13 | 0.34 | 0.031 | Y |
| **FOMUB–ARML** | 172 530 | 215 | 29 | 1.3 | 0.26 | 0.054 | Y |
| **AMUB–ARML** | 286 925 | 190 | 48 | 4.4 | 0.7 | 0.082 | N |
| **AMUB–FRML** | 431 966 | 204 | 142 | 17 | 0.37 | 0.0014 | N |
| **FO–ARML** | 796 081 | 201 | 1 | 3.5 | 0.42 | 0.14 | Y |
| **PAULI–CS** | 820 037 | 63 | 0.0082 | 1.1 | 0.14 | 0.013 | Y |
| **FO–FRML** | *1 057 832 | – | – | – | – | – | Y |
| **SGQT** | *1 175 629 | – | – | – | – | – | N |
| **FOMUB–FRML** | *2 251 263 | – | – | – | – | – | Y |
| **FMUB–FRLS** | *2 785 292 | – | – | – | – | – | Y |
| **FMUB–FRML** | *2 788 524 | – | – | – | – | – | Y |
| **MUB–FRML** | *2 793 700 | – | – | – | – | – | N |
| **FMUB–PPI** | *2 847 883 | – | – | – | – | – | Y |
| **FMUB–CS** | *3 551 649 | – | – | – | – | – | Y |

# 2 Random mixed states by partial tracing (rank-2) test

## 2.1 1 qubit

Table 13: Random mixed states by partial tracing (rank-2) test, 1 qubit, $F_B = 90\%$

| | $N_B$ | $M_B$ | $T_{P,B}$, sec | $T_{E,B}$, sec | $\eta_B$ | $O_B$ |
|---|---|---|---|---|---|---|
| **Lower bound** | 59 | – | – | – | 1 | – |
| **FMUB–FRLS** | *47 | – | – | – | – | – |
| **FMUB–PPI** | *47 | – | – | – | – | – |
| **MUB–FRML** | *48 | – | – | – | – | – |
| **FMUB–FRML** | *48 | – | – | – | – | – |
| **FMUB–TRML** | *48 | – | – | – | – | – |
| **AMUB–FRML** | *50 | – | – | – | – | – |
| **AMUB–ARML** | 155 | 5 | 0.94 | 0.017 | 0.44 | 0.0061 |
| **FMUB–CS** | 158 | 3 | 0.00044 | 0.59 | 0.41 | 0.012 |
| **MUB–ARML** | 214 | 3 | 0.00043 | 0.0087 | 0.37 | 0.042 |
| **FMUB–ARML** | 214 | 3 | 0.00073 | 0.013 | 0.37 | 0.042 |
| **PAULI–CS** | 3 755 | 3 | 0.00035 | 0.66 | 0.017 | 0 |

Table 14: Random mixed states by partial tracing (rank-2) test, 1 qubit, $F_B = 99\%$

| | $N_B$ | $M_B$ | $T_{P,B}$, sec | $T_{E,B}$, sec | $\eta_B$ | $O_B$ |
|---|---|---|---|---|---|---|
| **Lower bound** | 586 | – | – | – | 1 | – |
| **AMUB–FRML** | 750 | 11 | 0.021 | 0.0087 | 0.85 | 0.017 |
| **AMUB–ARML** | 989 | 12 | 1 | 0.037 | 0.72 | 0.032 |
| **MUB–FRML** | 1 109 | 3 | 0.00028 | 0.0031 | 0.65 | 0.03 |
| **FMUB–FRML** | 1 109 | 3 | 0.00044 | 0.0039 | 0.65 | 0.03 |
| **FMUB–TRML** | 1 109 | 3 | 0.00043 | 0.0047 | 0.65 | 0.03 |
| **FMUB–FRLS** | 1 110 | 3 | 0.00045 | 0.53 | 0.65 | 0.03 |
| **FMUB–PPI** | 1 110 | 3 | 0.00032 | 0.00053 | 0.65 | 0.03 |
| **MUB–ARML** | 2 735 | 3 | 0.00048 | 0.016 | 0.34 | 0.096 |
| **FMUB–ARML** | 2 735 | 3 | 0.00071 | 0.022 | 0.34 | 0.096 |
| **FMUB–CS** | 2 936 | 3 | 0.00042 | 0.58 | 0.31 | 0.057 |
| **PAULI–CS** | 150 126 | 3 | 0.00035 | 0.67 | 0.0076 | 0.0076 |

Table 15: Random mixed states by partial tracing (rank-2) test, 1 qubit, $F_B = 99.9\%$

| | $N_B$ | $M_B$ | $T_{P,B}$, sec | $T_{E,B}$, sec | $\eta_B$ | $O_B$ |
|---|---|---|---|---|---|---|
| **Lower bound** | 5 861 | – | – | – | 1 | – |
| **AMUB–FRML** | 6 332 | 58 | 0.2 | 0.013 | 0.97 | 0.0078 |
| **AMUB–ARML** | 6 630 | 59 | 1.1 | 0.093 | 0.95 | 0.011 |
| **MUB–FRML** | 10 126 | 3 | 0.00031 | 0.0033 | 0.62 | 0.037 |
| **FMUB–FRML** | 10 126 | 3 | 0.00046 | 0.0039 | 0.62 | 0.037 |
| **FMUB–TRML** | 10 126 | 3 | 0.00045 | 0.0049 | 0.62 | 0.037 |
| **FMUB–FRLS** | 10 126 | 3 | 0.00041 | 0.53 | 0.62 | 0.036 |
| **FMUB–PPI** | 10 126 | 3 | 0.00033 | 0.00059 | 0.62 | 0.036 |
| **MUB–ARML** | 18 008 | 3 | 0.00046 | 0.027 | 0.32 | 0.052 |
| **FMUB–ARML** | 18 008 | 3 | 0.00072 | 0.037 | 0.32 | 0.052 |
| **FMUB–CS** | 31 718 | 3 | 0.00042 | 0.58 | 0.26 | 0.05 |
| **PAULI–CS** | *1 142 951 | – | – | – | – | – |

Table 16: Random mixed states by partial tracing (rank-2) test, 1 qubit, $F_B = 99.99\%$

| | $N_B$ | $M_B$ | $T_{P,B}$, sec | $T_{E,B}$, sec | $\eta_B$ | $O_B$ |
|---|---|---|---|---|---|---|
| **Lower bound** | 58 610 | – | – | – | 1 | – |
| **AMUB–FRML** | 58 516 | 124 | 0.5 | 0.021 | 1 | 0.0027 |
| **AMUB–ARML** | 58 798 | 124 | 3.2 | 0.15 | 1 | 0.0022 |
| **MUB–FRML** | 106 277 | 3 | 0.00028 | 0.0031 | 0.5 | 0.037 |
| **FMUB–FRML** | 106 277 | 3 | 0.00043 | 0.0039 | 0.5 | 0.037 |
| **FMUB–TRML** | 106 277 | 3 | 0.0005 | 0.005 | 0.5 | 0.037 |
| **FMUB–FRLS** | 106 277 | 3 | 0.00043 | 0.54 | 0.5 | 0.037 |
| **FMUB–PPI** | 106 277 | 3 | 0.00034 | 0.00053 | 0.5 | 0.037 |
| **MUB–ARML** | 114 501 | 3 | 0.00039 | 0.033 | 0.3 | 0.042 |
| **FMUB–ARML** | 114 501 | 3 | 0.00069 | 0.049 | 0.3 | 0.042 |
| **FMUB–CS** | 281 587 | 3 | 0.0004 | 0.59 | 0.24 | 0.042 |
| **PAULI–CS** | *1 343 850 | – | – | – | – | – |

## 2.2 2 qubits

Table 17: Random mixed states by partial tracing (rank-2) test, 2 qubits, $F_B = 90\%$

| | $N_B$ | $M_B$ | $T_{P,B}$, sec | $T_{E,B}$, sec | $\eta_B$ | $O_B$ | FM |
|---:|---:|---:|---:|---:|---:|---:|---:|
| **Lower bound** | 180 | – | – | – | 1 | – | – |
| **FMUB–TRML** | 285 | 9 | 0.00087 | 0.011 | 0.72 | 0.03 | Y |
| **MUB–ARML** | 378 | 5 | 0.00054 | 0.014 | 0.59 | 0.024 | N |
| **AMUB–ARML** | 381 | 8 | 0.037 | 0.073 | 0.61 | 0.027 | N |
| **FMUB–ARML** | 399 | 9 | 0.0011 | 0.022 | 0.55 | 0.023 | Y |
| **FMUB–CS** | 411 | 9 | 0.00083 | 0.59 | 0.52 | 0.017 | Y |
| **AMUB–FRML** | 416 | 8 | 0.07 | 0.089 | 0.52 | 0.0042 | N |
| **FOMUB–ARML** | 456 | 15 | 0.086 | 0.094 | 0.54 | 0.039 | Y |
| **MUB–FRML** | 468 | 5 | 0.00061 | 0.023 | 0.45 | 0.005 | N |
| **FOMUB–FRML** | 491 | 15 | 0.27 | 0.32 | 0.48 | 0.012 | Y |
| **FMUB–FRML** | 510 | 9 | 0.00055 | 0.047 | 0.43 | 0.0035 | Y |
| **FMUB–FRLS** | 616 | 9 | 0.00094 | 0.47 | 0.35 | 0.0035 | Y |
| **FMUB–PPI** | 642 | 9 | 0.00062 | 0.00056 | 0.33 | 0.0026 | Y |
| **FO–ARML** | 1 861 | 25 | 177 | 0.23 | 0.21 | 0.052 | Y |
| **FO–FRML** | 2 275 | 30 | 97 | 0.35 | 0.16 | 0.032 | Y |
| **PAULI–CS** | 13 558 | 15 | 0.0018 | 0.78 | 0.022 | 0.024 | Y |

Table 18: Random mixed states by partial tracing (rank-2) test, 2 qubits, $F_B = 99\%$

| | $N_B$ | $M_B$ | $T_{P,B}$, sec | $T_{E,B}$, sec | $\eta_B$ | $O_B$ | FM |
|---:|---:|---:|---:|---:|---:|---:|---:|
| **Lower bound** | 1 804 | – | – | – | 1 | – | – |
| **FMUB–TRML** | 3 367 | 9 | 0.00086 | 0.011 | 0.61 | 0.026 | Y |
| **MUB–ARML** | 3 568 | 5 | 0.00054 | 0.025 | 0.56 | 0.05 | N |
| **FMUB–ARML** | 3 856 | 9 | 0.0011 | 0.037 | 0.55 | 0.037 | Y |
| **FOMUB–ARML** | 3 986 | 50 | 0.7 | 0.16 | 0.59 | 0.041 | Y |
| **AMUB–ARML** | 4 324 | 48 | 0.93 | 0.16 | 0.61 | 0.047 | N |
| **AMUB–FRML** | 6 850 | 60 | 1.7 | 0.24 | 0.34 | 0.012 | N |
| **FO–ARML** | 7 695 | 61 | 182 | 0.28 | 0.35 | 0.025 | Y |
| **FOMUB–FRML** | 13 475 | 82 | 7.1 | 1.3 | 0.22 | 0.001 | Y |
| **FMUB–CS** | 17 178 | 9 | 0.00087 | 0.44 | 0.2 | 0.06 | Y |
| **FO–FRML** | 17 834 | 85 | 110 | 0.52 | 0.17 | 0.01 | Y |
| **MUB–FRML** | 36 589 | 5 | 0.0006 | 0.094 | 0.066 | 0.0023 | N |
| **FMUB–FRML** | 36 915 | 9 | 0.00056 | 0.23 | 0.069 | 0.0011 | Y |
| **FMUB–FRLS** | 48 837 | 9 | 0.00091 | 0.48 | 0.051 | 0.00062 | Y |
| **FMUB–PPI** | 51 126 | 9 | 0.00063 | 0.00054 | 0.048 | 0.00058 | Y |
| **PAULI–CS** | 116 837 | 15 | 0.0019 | 0.83 | 0.03 | 0.059 | Y |

Table 19: Random mixed states by partial tracing (rank-2) test, 2 qubits, $F_B = 99.9\%$

| | $N_B$ | $M_B$ | $T_{P,B}$, sec | $T_{E,B}$, sec | $\eta_B$ | $O_B$ | FM |
|---:|---:|---:|---:|---:|---:|---:|---:|
| **Lower bound** | 18 036 | – | – | – | 1 | – | – |
| **FMUB–TRML** | 33 783 | 9 | 0.00086 | 0.0092 | 0.62 | 0.022 | Y |
| **MUB–ARML** | 34 762 | 5 | 0.00054 | 0.038 | 0.45 | 0.046 | N |
| **FMUB–ARML** | 37 554 | 9 | 0.0011 | 0.057 | 0.46 | 0.037 | Y |
| **FOMUB–ARML** | 37 717 | 119 | 2.5 | 0.21 | 0.58 | 0.039 | Y |
| **AMUB–ARML** | 46 546 | 120 | 3.3 | 0.22 | 0.59 | 0.057 | N |
| **AMUB–FRML** | 77 273 | 137 | 6.1 | 0.57 | 0.32 | 0.018 | N |
| **FO–ARML** | 86 968 | 134 | 194 | 0.5 | 0.35 | 0.055 | Y |
| **FOMUB–FRML** | 217 640 | 180 | 20 | 2 | 0.16 | 0.013 | Y |
| **FO–FRML** | 353 999 | 176 | 166 | 1.4 | 0.097 | 0.05 | Y |
| **PAULI–CS** | 859 369 | 15 | 0.0019 | 0.81 | 0.039 | 0.039 | Y |
| **FMUB–CS** | *1 156 881 | – | – | – | – | – | Y |
| **FMUB–FRML** | *1 612 140 | – | – | – | – | – | Y |
| **MUB–FRML** | *1 619 547 | – | – | – | – | – | N |
| **FMUB–FRLS** | *1 765 515 | – | – | – | – | – | Y |
| **FMUB–PPI** | *1 782 349 | – | – | – | – | – | Y |

Table 20: Random mixed states by partial tracing (rank-2) test, 2 qubits, $F_B = 99.99\%$

| | $N_B$ | $M_B$ | $T_{P,B}$, sec | $T_{E,B}$, sec | $\eta_B$ | $O_B$ | FM |
|---:|---:|---:|---:|---:|---:|---:|---:|
| **Lower bound** | 180 355 | – | – | – | 1 | – | – |
| **FMUB–TRML** | 340 894 | 9 | 0.00086 | 0.0085 | 0.62 | 0.022 | Y |
| **MUB–ARML** | 360 923 | 5 | 0.00054 | 0.045 | 0.26 | 0.038 | N |
| **FOMUB–ARML** | 374 387 | 199 | 5.4 | 0.25 | 0.55 | 0.05 | Y |
| **FMUB–ARML** | 378 165 | 9 | 0.0012 | 0.063 | 0.29 | 0.034 | Y |
| **AMUB–ARML** | 414 549 | 191 | 6.9 | 0.31 | 0.62 | 0.038 | N |
| **FO–ARML** | 887 248 | 204 | 229 | 0.67 | 0.34 | 0.052 | Y |
| **AMUB–FRML** | 895 449 | 216 | 13 | 0.92 | 0.29 | 0.013 | N |
| **PAULI–CS** | *1 165 365 | – | – | – | – | – | Y |
| **FOMUB–FRML** | *1 205 477 | – | – | – | – | – | Y |
| **FO–FRML** | *1 277 361 | – | – | – | – | – | Y |
| **FMUB–CS** | *2 334 153 | – | – | – | – | – | Y |
| **MUB–FRML** | *2 708 766 | – | – | – | – | – | N |
| **FMUB–FRML** | *2 716 723 | – | – | – | – | – | Y |
| **FMUB–PPI** | *2 727 413 | – | – | – | – | – | Y |
| **FMUB–FRLS** | *2 728 501 | – | – | – | – | – | Y |

### 2.3 3 qubits

Table 21: Random mixed states by partial tracing (rank-2) test, 3 qubits, $F_B = 90\%$

| | $N_B$ | $M_B$ | $T_{P,B}$, sec | $T_{E,B}$, sec | $\eta_B$ | $O_B$ | FM |
|---:|---:|---:|---:|---:|---:|---:|:---:|
| **Lower bound** | 387 | – | – | – | 1 | – | – |
| **MUB–ARML** | *167 | – | – | – | – | – | N |
| **FMUB–TRML** | *257 | – | – | – | – | – | Y |
| **FOMUB–ARML** | *383 | – | – | – | – | – | Y |
| **FMUB–ARML** | *386 | – | – | – | – | – | Y |
| **AMUB–ARML** | *757 | – | – | – | – | – | N |
| **AMUB–FRML** | 1 319 | 24 | 2.4 | 1.4 | 0.31 | 0.016 | N |
| **FMUB–CS** | 1 648 | 27 | 0.002 | 0.71 | 0.3 | 0.0034 | Y |
| **MUB–FRML** | 1 836 | 9 | 0.00057 | 0.13 | 0.22 | 0.0061 | N |
| **FOMUB–FRML** | 1 873 | 42 | 4 | 7.3 | 0.22 | 0.011 | Y |
| **FMUB–FRML** | 1 947 | 27 | 0.0018 | 0.4 | 0.21 | 0.012 | Y |
| **FO–ARML** | 2 365 | 31 | 0.98 | 1.1 | 0.31 | 0.058 | Y |
| **FO–FRML** | 2 922 | 37 | 268 | 3.3 | 0.17 | 0.02 | Y |
| **FMUB–FRLS** | 2 965 | 27 | 0.0019 | 0.47 | 0.14 | 0.0091 | Y |
| **FMUB–PPI** | 3 708 | 27 | 0.0018 | 0.0026 | 0.11 | 0.0071 | Y |
| **PAULI–CS** | 24 508 | 63 | 0.0082 | 1.1 | 0.021 | 0.02 | Y |

Table 22: Random mixed states by partial tracing (rank-2) test, 3 qubits, $F_B = 99\%$

| | $N_B$ | $M_B$ | $T_{P,B}$, sec | $T_{E,B}$, sec | $\eta_B$ | $O_B$ | FM |
|---:|---:|---:|---:|---:|---:|---:|:---:|
| **Lower bound** | 3 868 | – | – | – | 1 | – | – |
| **MUB–ARML** | 5 988 | 9 | 0.001 | 0.061 | 0.67 | 0.034 | N |
| **FMUB–TRML** | 6 001 | 27 | 0.003 | 0.031 | 0.71 | 0.011 | Y |
| **FMUB–ARML** | 6 450 | 27 | 0.0019 | 0.062 | 0.64 | 0.023 | Y |
| **FOMUB–ARML** | 6 858 | 72 | 1.6 | 1.6 | 0.59 | 0.045 | Y |
| **AMUB–ARML** | 9 771 | 71 | 4.2 | 1.5 | 0.65 | 0.065 | N |
| **FO–ARML** | 14 218 | 78 | 1 | 2.3 | 0.49 | 0.1 | Y |
| **AMUB–FRML** | 15 375 | 87 | 37 | 12 | 0.32 | 0.015 | N |
| **FO–FRML** | 30 208 | 101 | 522 | 8 | 0.16 | 0.014 | Y |
| **FMUB–CS** | 97 437 | 27 | 0.002 | 0.52 | 0.062 | 0.0099 | Y |
| **FOMUB–FRML** | 107 701 | 192 | 506 | 385 | 0.04 | 0.0042 | Y |
| **PAULI–CS** | 155 921 | 63 | 0.0082 | 1.1 | 0.041 | 0.05 | Y |
| **FMUB–FRML** | 161 345 | 27 | 0.0018 | 1.7 | 0.026 | 0.0093 | Y |
| **MUB–FRML** | 164 625 | 9 | 0.00053 | 0.68 | 0.025 | 0.008 | N |
| **FMUB–FRLS** | 276 815 | 27 | 0.0019 | 0.48 | 0.015 | 0.0031 | Y |
| **FMUB–PPI** | 337 607 | 27 | 0.0018 | 0.0026 | 0.012 | 0.0055 | Y |

Table 23: Random mixed states by partial tracing (rank-2) test, 3 qubits, $F_B = 99.9\%$

| | $N_B$ | $M_B$ | $T_{P,B}$, sec | $T_{E,B}$, sec | $\eta_B$ | $O_B$ | FM |
|---|---|---|---|---|---|---|---|
| **Lower bound** | 38 681 | – | – | – | 1 | – | – |
| **MUB–ARML** | 55 604 | 9 | 0.00099 | 0.076 | 0.57 | 0.038 | N |
| **FMUB–TRML** | 57 833 | 27 | 0.0033 | 0.026 | 0.72 | 0.0082 | Y |
| **FMUB–ARML** | 60 677 | 27 | 0.0019 | 0.066 | 0.52 | 0.021 | Y |
| **FOMUB–ARML** | 62 941 | 167 | 21 | 6.1 | 0.47 | 0.038 | Y |
| **AMUB–ARML** | 92 580 | 150 | 40 | 7.2 | 0.65 | 0.062 | N |
| **AMUB–FRML** | 141 855 | 165 | 180 | 35 | 0.33 | 0.012 | N |
| **FO–ARML** | 147 916 | 150 | 1 | 6.8 | 0.48 | 0.069 | Y |
| **FO–FRML** | 337 222 | 175 | 1 417 | 18 | 0.15 | 0.014 | Y |
| **PAULI–CS** | 1 215 947 | 63 | 0.0085 | 1.1 | 0.05 | 0.043 | Y |
| **FOMUB–FRML** | 7 270 918 | 367 | 9 828 | 4 927 | 0.0068 | 0.0066 | Y |
| **FMUB–CS** | 9 445 112 | 27 | 0.0019 | 0.55 | 0.0068 | 0.003 | Y |
| **MUB–FRML** | *12 623 083 | – | – | – | – | – | N |
| **FMUB–FRML** | *12 704 198 | – | – | – | – | – | Y |
| **FMUB–FRLS** | *15 353 412 | – | – | – | – | – | Y |
| **FMUB–PPI** | *16 148 565 | – | – | – | – | – | Y |

Table 24: Random mixed states by partial tracing (rank-2) test, 3 qubits, $F_B = 99.99\%$

| | $N_B$ | $M_B$ | $T_{P,B}$, sec | $T_{E,B}$, sec | $\eta_B$ | $O_B$ | FM |
|---|---|---|---|---|---|---|---|
| **Lower bound** | 386 807 | – | – | – | 1 | – | – |
| **MUB–ARML** | 536 526 | 9 | 0.001 | 0.081 | 0.35 | 0.028 | N |
| **FMUB–TRML** | 577 409 | 27 | 0.0031 | 0.025 | 0.72 | 0.012 | Y |
| **FMUB–ARML** | 602 455 | 27 | 0.0018 | 0.059 | 0.38 | 0.023 | Y |
| **FOMUB–ARML** | 630 833 | 275 | 87 | 11 | 0.35 | 0.034 | Y |
| **AMUB–ARML** | 863 149 | 229 | 145 | 16 | 0.68 | 0.07 | N |
| **AMUB–FRML** | 1 466 307 | 247 | 555 | 67 | 0.32 | 0.0092 | N |
| **FO–ARML** | 1 528 936 | 221 | 1 | 16 | 0.48 | 0.063 | Y |
| **FO–FRML** | 3 570 553 | 247 | 2 965 | 31 | 0.14 | 0.012 | Y |
| **PAULI–CS** | *10 269 072 | – | – | – | – | – | Y |
| **FOMUB–FRML** | *21 890 735 | – | – | – | – | – | Y |
| **FMUB–CS** | *25 562 993 | – | – | – | – | – | Y |
| **FMUB–FRML** | *26 555 178 | – | – | – | – | – | Y |
| **MUB–FRML** | *26 681 907 | – | – | – | – | – | N |
| **FMUB–FRLS** | *27 097 716 | – | – | – | – | – | Y |
| **FMUB–PPI** | *27 176 645 | – | – | – | – | – | Y |

# 3 Random mixed states by partial tracing (full-rank) test

## 3.1 1 qubit

Table 25: Random mixed states by partial tracing (full-rank) test, 1 qubit, $F_B = 90\%$

| | $N_B$ | $M_B$ | $T_{P,B}$, sec | $T_{E,B}$, sec | $\eta_B$ | $O_B$ |
|---:|---:|---:|---:|---:|---:|---:|
| **Lower bound** | 59 | – | – | – | 1 | – |
| **MUB–FRML** | *62 | – | – | – | – | – |
| **FMUB–FRML** | *62 | – | – | – | – | – |
| **FMUB–TRML** | *62 | – | – | – | – | – |
| **AMUB–FRML** | *63 | – | – | – | – | – |
| **FMUB–FRLS** | *65 | – | – | – | – | – |
| **FMUB–PPI** | *65 | – | – | – | – | – |
| **AMUB–ARML** | 155 | 5 | 0.94 | 0.018 | 0.44 | 0.0047 |
| **FMUB–CS** | 165 | 3 | 0.00036 | 0.52 | 0.4 | 0.012 |
| **MUB–ARML** | 225 | 3 | 0.00046 | 0.0099 | 0.37 | 0.039 |
| **FMUB–ARML** | 225 | 3 | 0.00051 | 0.0094 | 0.37 | 0.039 |
| **PAULI–CS** | 3 654 | 3 | 0.00039 | 0.65 | 0.017 | 0 |

Table 26: Random mixed states by partial tracing (full-rank) test, 1 qubit, $F_B = 99\%$

| | $N_B$ | $M_B$ | $T_{P,B}$, sec | $T_{E,B}$, sec | $\eta_B$ | $O_B$ |
|---:|---:|---:|---:|---:|---:|---:|
| **Lower bound** | 586 | – | – | – | 1 | – |
| **AMUB–FRML** | 731 | 11 | 0.022 | 0.009 | 0.85 | 0.013 |
| **AMUB–ARML** | 860 | 11 | 0.99 | 0.036 | 0.73 | 0.023 |
| **MUB–FRML** | 994 | 3 | 0.00028 | 0.0031 | 0.67 | 0.028 |
| **FMUB–FRML** | 994 | 3 | 0.00031 | 0.003 | 0.67 | 0.028 |
| **FMUB–TRML** | 994 | 3 | 0.00031 | 0.003 | 0.67 | 0.028 |
| **FMUB–FRLS** | 1 015 | 3 | 0.00034 | 0.41 | 0.66 | 0.027 |
| **FMUB–PPI** | 1 015 | 3 | 0.00031 | 0.00051 | 0.67 | 0.027 |
| **MUB–ARML** | 2 739 | 3 | 0.0005 | 0.016 | 0.33 | 0.089 |
| **FMUB–ARML** | 2 739 | 3 | 0.0005 | 0.017 | 0.33 | 0.089 |
| **FMUB–CS** | 2 758 | 3 | 0.00037 | 0.5 | 0.31 | 0.069 |
| **PAULI–CS** | 133 933 | 3 | 0.00037 | 0.66 | 0.0081 | 0.036 |

Table 27: Random mixed states by partial tracing (full-rank) test, 1 qubit, $F_B = 99.9\%$

| | $N_B$ | $M_B$ | $T_{P,B}$, sec | $T_{E,B}$, sec | $\eta_B$ | $O_B$ |
|---|---|---|---|---|---|---|
| **Lower bound** | 5 861 | – | – | – | 1 | – |
| **AMUB–FRML** | 6 115 | 57 | 0.19 | 0.013 | 0.95 | 0.0095 |
| **AMUB–ARML** | 6 333 | 58 | 1.1 | 0.086 | 0.93 | 0.012 |
| **MUB–FRML** | 11 637 | 3 | 0.00029 | 0.0032 | 0.58 | 0.033 |
| **FMUB–FRML** | 11 637 | 3 | 0.00031 | 0.0029 | 0.58 | 0.033 |
| **FMUB–TRML** | 11 637 | 3 | 0.00031 | 0.0029 | 0.58 | 0.033 |
| **FMUB–FRLS** | 11 704 | 3 | 0.00034 | 0.41 | 0.58 | 0.033 |
| **FMUB–PPI** | 11 714 | 3 | 0.00032 | 0.00057 | 0.58 | 0.033 |
| **MUB–ARML** | 19 430 | 3 | 0.0005 | 0.028 | 0.31 | 0.058 |
| **FMUB–ARML** | 19 430 | 3 | 0.00053 | 0.029 | 0.31 | 0.058 |
| **FMUB–CS** | 31 857 | 3 | 0.00038 | 0.49 | 0.25 | 0.07 |
| **PAULI–CS** | *1 197 040 | – | – | – | – | – |

Table 28: Random mixed states by partial tracing (full-rank) test, 1 qubit, $F_B = 99.99\%$

| | $N_B$ | $M_B$ | $T_{P,B}$, sec | $T_{E,B}$, sec | $\eta_B$ | $O_B$ |
|---|---|---|---|---|---|---|
| **Lower bound** | 58 610 | – | – | – | 1 | – |
| **AMUB–FRML** | 60 176 | 125 | 0.51 | 0.017 | 0.99 | 0.0041 |
| **AMUB–ARML** | 60 994 | 126 | 3.1 | 0.16 | 0.99 | 0.0043 |
| **MUB–FRML** | 134 940 | 3 | 0.00029 | 0.0033 | 0.42 | 0.046 |
| **FMUB–FRML** | 134 940 | 3 | 0.00029 | 0.0029 | 0.42 | 0.046 |
| **FMUB–TRML** | 134 940 | 3 | 0.00029 | 0.0029 | 0.42 | 0.046 |
| **FMUB–FRLS** | 134 940 | 3 | 0.00033 | 0.42 | 0.42 | 0.046 |
| **FMUB–PPI** | 134 940 | 3 | 0.00031 | 0.00048 | 0.42 | 0.046 |
| **MUB–ARML** | 160 823 | 3 | 0.00044 | 0.039 | 0.28 | 0.051 |
| **FMUB–ARML** | 160 823 | 3 | 0.00054 | 0.035 | 0.28 | 0.051 |
| **FMUB–CS** | 327 330 | 3 | 0.00037 | 0.5 | 0.2 | 0.053 |
| **PAULI–CS** | *1 447 123 | – | – | – | – | – |

### 3.2 2 qubits

Table 29: Random mixed states by partial tracing (full-rank) test, 2 qubits, $F_B = 90\%$

| | $N_B$ | $M_B$ | $T_{P,B}$, sec | $T_{E,B}$, sec | $\eta_B$ | $O_B$ | FM |
|---|---|---|---|---|---|---|---|
| **Lower bound** | 312 | – | – | – | 1 | – | – |
| **MUB–FRML** | *143 | – | – | – | – | – | N |
| **AMUB–FRML** | *146 | – | – | – | – | – | N |
| **FMUB–FRML** | *291 | – | – | – | – | – | Y |
| **FMUB–TRML** | *291 | – | – | – | – | – | Y |
| **FMUB–FRLS** | *341 | – | – | – | – | – | Y |
| **FMUB–PPI** | *346 | – | – | – | – | – | Y |
| **FOMUB–FRML** | *704 | – | – | – | – | – | Y |
| **FMUB–CS** | *759 | – | – | – | – | – | Y |
| **AMUB–ARML** | 1 187 | 14 | 0.41 | 0.25 | 0.36 | 0.012 | N |
| **MUB–ARML** | 1 277 | 5 | 0.00074 | 0.047 | 0.33 | 0.0063 | N |
| **FMUB–ARML** | 2 013 | 9 | 0.0012 | 0.058 | 0.21 | 0 | Y |
| **FOMUB–ARML** | 2 692 | 41 | 1.1 | 0.35 | 0.17 | 0.00086 | Y |
| **FO–FRML** | 3 323 | 40 | 108 | 0.78 | 0.15 | 0.028 | Y |
| **FO–ARML** | 5 781 | 53 | 194 | 0.92 | 0.084 | 0.0056 | Y |
| **PAULI–CS** | 33 424 | 15 | 0.0023 | 0.95 | 0.01 | 0.0033 | Y |

Table 30: Random mixed states by partial tracing (full-rank) test, 2 qubits, $F_B = 99\%$

| | $N_B$ | $M_B$ | $T_{P,B}$, sec | $T_{E,B}$, sec | $\eta_B$ | $O_B$ | FM |
|---|---|---|---|---|---|---|---|
| **Lower bound** | 3 124 | – | – | – | 1 | – | – |
| **AMUB–FRML** | 8 842 | 67 | 0.76 | 0.083 | 0.55 | 0.046 | N |
| **MUB–FRML** | 10 061 | 5 | 0.00077 | 0.0081 | 0.45 | 0.02 | N |
| **FMUB–FRML** | 14 593 | 9 | 0.0007 | 0.067 | 0.34 | 0.03 | Y |
| **FMUB–TRML** | 14 593 | 9 | 0.0007 | 0.067 | 0.34 | 0.03 | Y |
| **FOMUB–FRML** | 15 580 | 88 | 7.7 | 0.72 | 0.33 | 0.048 | Y |
| **FMUB–FRLS** | 15 829 | 9 | 0.00093 | 0.46 | 0.32 | 0.026 | Y |
| **FMUB–PPI** | 16 172 | 9 | 0.0006 | 0.00053 | 0.31 | 0.029 | Y |
| **AMUB–ARML** | 21 500 | 95 | 9.9 | 1.4 | 0.29 | 0.067 | N |
| **FMUB–CS** | 28 781 | 9 | 0.00092 | 0.53 | 0.19 | 0.03 | Y |
| **MUB–ARML** | 34 698 | 5 | 0.00077 | 0.1 | 0.2 | 0.055 | N |
| **FO–FRML** | 65 133 | 125 | 152 | 0.76 | 0.087 | 0.026 | Y |
| **FMUB–ARML** | 105 060 | 9 | 0.0012 | 0.11 | 0.073 | 0.016 | Y |
| **FOMUB–ARML** | 550 338 | 213 | 13 | 1 | 0.016 | 0 | Y |
| **FO–ARML** | 1 688 307 | 224 | 756 | 13 | 0.0052 | 0.014 | Y |
| **PAULI–CS** | 1 803 478 | 15 | 0.0023 | 0.95 | 0.0026 | 0.0013 | Y |

Table 31: Random mixed states by partial tracing (full-rank) test, 2 qubits, $F_B = 99.9\%$

| | $N_B$ | $M_B$ | $T_{P,B}$, sec | $T_{E,B}$, sec | $\eta_B$ | $O_B$ | FM |
|---|---|---|---|---|---|---|---|
| **Lower bound** | 31 245 | – | – | – | 1 | – | – |
| **AMUB–FRML** | 62 112 | 129 | 1.6 | 0.08 | 0.64 | 0.02 | N |
| **AMUB–ARML** | 153 895 | 159 | 31 | 3.5 | 0.4 | 0.1 | N |
| **MUB–FRML** | 160 266 | 5 | 0.00073 | 0.0064 | 0.35 | 0.061 | N |
| **FMUB–FRML** | 233 051 | 9 | 0.00067 | 0.068 | 0.25 | 0.069 | Y |
| **FMUB–TRML** | 233 051 | 9 | 0.00067 | 0.068 | 0.25 | 0.069 | Y |
| **FMUB–FRLS** | 262 741 | 9 | 0.00091 | 0.46 | 0.23 | 0.057 | Y |
| **FMUB–PPI** | 265 894 | 9 | 0.00061 | 0.00055 | 0.23 | 0.057 | Y |
| **FOMUB–FRML** | 268 040 | 188 | 20 | 0.84 | 0.24 | 0.073 | Y |
| **FMUB–CS** | 572 506 | 9 | 0.00092 | 0.52 | 0.13 | 0.091 | Y |
| **MUB–ARML** | 666 698 | 5 | 0.00074 | 0.13 | 0.15 | 0.13 | N |
| **FMUB–ARML** | 2 005 212 | 9 | 0.0012 | 0.14 | 0.058 | 0.18 | Y |
| **FO–FRML** | 3 446 412 | 246 | 328 | 4.1 | 0.02 | 0.016 | Y |
| **FO–ARML** | *16 610 646 | – | – | – | – | – | Y |
| **PAULI–CS** | *19 125 276 | – | – | – | – | – | Y |
| **FOMUB–ARML** | *40 463 638 | – | – | – | – | – | Y |

Table 32: Random mixed states by partial tracing (full-rank) test, 2 qubits, $F_B = 99.99\%$

| | $N_B$ | $M_B$ | $T_{P,B}$, sec | $T_{E,B}$, sec | $\eta_B$ | $O_B$ | FM |
|---|---|---|---|---|---|---|---|
| **Lower bound** | 312 447 | – | – | – | 1 | – | – |
| **AMUB–FRML** | 591 657 | 203 | 2.9 | 0.11 | 0.64 | 0.023 | N |
| **AMUB–ARML** | 758 254 | 211 | 67 | 7.6 | 0.49 | 0.043 | N |
| **MUB–FRML** | 2 066 031 | 5 | 0.00077 | 0.0057 | 0.28 | 0.071 | N |
| **FMUB–FRML** | 3 049 758 | 9 | 0.00068 | 0.073 | 0.2 | 0.084 | Y |
| **FMUB–TRML** | 3 049 758 | 9 | 0.00068 | 0.073 | 0.2 | 0.084 | Y |
| **FMUB–PPI** | 3 554 953 | 9 | 0.00061 | 0.00052 | 0.18 | 0.074 | Y |
| **FMUB–FRLS** | 3 555 013 | 9 | 0.0009 | 0.46 | 0.18 | 0.075 | Y |
| **FOMUB–FRML** | 4 249 725 | 285 | 33 | 1.1 | 0.1 | 0.098 | Y |
| **MUB–ARML** | 5 207 085 | 5 | 0.00074 | 0.15 | 0.12 | 0.1 | N |
| **FMUB–CS** | 8 325 077 | 9 | 0.00094 | 0.53 | 0.087 | 0.1 | Y |
| **FMUB–ARML** | *10 815 451 | – | – | – | – | – | Y |
| **FO–FRML** | *17 364 377 | – | – | – | – | – | Y |
| **FO–ARML** | *20 227 652 | – | – | – | – | – | Y |
| **PAULI–CS** | *23 494 630 | – | – | – | – | – | Y |
| **FOMUB–ARML** | *67 306 094 | – | – | – | – | – | Y |

### 3.3 3 qubits

Table 33: Random mixed states by partial tracing (full-rank) test, 3 qubits, $F_B = 90\%$

| | $N_B$ | $M_B$ | $T_{P,B}$, sec | $T_{E,B}$, sec | $\eta_B$ | $O_B$ | FM |
|---:|---:|---:|---:|---:|---:|---:|---:|
| **Lower bound** | 1 857 | – | – | – | 1 | – | – |
| **MUB–FRML** | *112 | – | – | – | – | – | N |
| **AMUB–FRML** | *201 | – | – | – | – | – | N |
| **FOMUB–FRML** | *1 148 | – | – | – | – | – | Y |
| **FMUB–FRML** | *1 170 | – | – | – | – | – | Y |
| **FMUB–TRML** | *1 170 | – | – | – | – | – | Y |
| **FMUB–FRLS** | *1 299 | – | – | – | – | – | Y |
| **FMUB–PPI** | *1 598 | – | – | – | – | – | Y |
| **FMUB–CS** | *2 331 | – | – | – | – | – | Y |
| **MUB–ARML** | *3 316 | – | – | – | – | – | N |
| **FO–FRML** | *6 255 | – | – | – | – | – | Y |
| **AMUB–ARML** | *6 335 | – | – | – | – | – | N |
| **FMUB–ARML** | 19 160 | 27 | 0.0028 | 0.78 | 0.12 | 0.0044 | Y |
| **FOMUB–ARML** | 32 968 | 137 | 166 | 105 | 0.075 | 0.0024 | Y |
| **FO–ARML** | 78 302 | 130 | 0.98 | 155 | 0.033 | 0.0044 | Y |
| **PAULI–CS** | 401 882 | 63 | 0.0056 | 0.83 | 0.0049 | 0.0032 | Y |

Table 34: Random mixed states by partial tracing (full-rank) test, 3 qubits, $F_B = 99\%$

| | $N_B$ | $M_B$ | $T_{P,B}$, sec | $T_{E,B}$, sec | $\eta_B$ | $O_B$ | FM |
|---:|---:|---:|---:|---:|---:|---:|---:|
| **Lower bound** | 18 569 | – | – | – | 1 | – | – |
| **AMUB–FRML** | 40 412 | 121 | 33 | 5.3 | 0.55 | 0.02 | N |
| **MUB–FRML** | 58 098 | 9 | 0.00065 | 0.08 | 0.4 | 0.0044 | N |
| **FMUB–FRML** | 105 039 | 27 | 0.0013 | 0.7 | 0.23 | 0.0072 | Y |
| **FMUB–TRML** | 105 039 | 27 | 0.0013 | 0.7 | 0.23 | 0.0072 | Y |
| **FMUB–FRLS** | 108 665 | 27 | 0.0023 | 0.56 | 0.22 | 0.0072 | Y |
| **FMUB–PPI** | 111 638 | 27 | 0.0017 | 0.0027 | 0.22 | 0.0086 | Y |
| **FOMUB–FRML** | 124 270 | 199 | 288 | 165 | 0.2 | 0.0095 | Y |
| **FMUB–CS** | 144 109 | 27 | 0.0027 | 0.57 | 0.17 | 0.0072 | Y |
| **MUB–ARML** | 146 532 | 9 | 0.0011 | 0.58 | 0.21 | 0.005 | N |
| **AMUB–ARML** | 272 951 | 188 | 3 137 | 653 | 0.14 | 0 | N |
| **FO–FRML** | 306 509 | 172 | 3 809 | 68 | 0.09 | 0.016 | Y |
| **FMUB–ARML** | 646 936 | 27 | 0.0025 | 1.2 | 0.055 | 0.0015 | Y |
| **FOMUB–ARML** | 2 707 908 | 332 | 1 855 | 514 | 0.014 | 0.00043 | Y |
| **FO–ARML** | 7 046 428 | 267 | 1 | 1 008 | 0.006 | 0.0015 | Y |
| **PAULI–CS** | 15 953 034 | 63 | 0.0055 | 0.82 | 0.0015 | 0 | Y |

Table 35: Random mixed states by partial tracing (full-rank) test, 3 qubits, $F_B = 99.9\%$

| | $N_B$ | $M_B$ | $T_{P,B}$, sec | $T_{E,B}$, sec | $\eta_B$ | $O_B$ | FM |
|---:|---:|---:|---:|---:|---:|---:|---:|
| **Lower bound** | 185 690 | – | – | – | 1 | – | – |
| **AMUB–FRML** | 439 161 | 205 | 106 | 11 | 0.52 | 0.022 | N |
| **MUB–FRML** | 1 197 954 | 9 | 0.0007 | 0.041 | 0.28 | 0.05 | N |
| **FMUB–FRML** | 2 391 759 | 27 | 0.0013 | 1.2 | 0.16 | 0.032 | Y |
| **FMUB–TRML** | 2 391 759 | 27 | 0.0013 | 1.2 | 0.16 | 0.032 | Y |
| **FMUB–FRLS** | 2 398 406 | 27 | 0.0022 | 0.57 | 0.15 | 0.048 | Y |
| **FMUB–PPI** | 2 419 468 | 27 | 0.0016 | 0.0028 | 0.15 | 0.047 | Y |
| **AMUB–ARML** | 3 069 798 | 273 | 14 718 | 2 452 | 0.17 | 0.056 | N |
| **FMUB–CS** | 3 733 351 | 27 | 0.0026 | 0.58 | 0.1 | 0.043 | Y |
| **MUB–ARML** | 3 818 905 | 9 | 0.0011 | 0.68 | 0.14 | 0.08 | N |
| **FO–FRML** | 9 496 329 | 276 | 15 619 | 204 | 0.045 | 0.054 | Y |
| **FOMUB–FRML** | 9 671 663 | 377 | 2 588 | 692 | 0.063 | 0.093 | Y |
| **FOMUB–ARML** | *23 033 115 | – | – | – | – | – | Y |
| **FO–ARML** | *24 238 669 | – | – | – | – | – | Y |
| **FMUB–ARML** | 36 526 642 | 27 | 0.0026 | 1.4 | 0.019 | 0.099 | Y |
| **PAULI–CS** | *165 463 605 | – | – | – | – | – | Y |

Table 36: Random mixed states by partial tracing (full-rank) test, 3 qubits, $F_B = 99.99\%$

| | $N_B$ | $M_B$ | $T_{P,B}$, sec | $T_{E,B}$, sec | $\eta_B$ | $O_B$ | FM |
|---:|---:|---:|---:|---:|---:|---:|---:|
| **Lower bound** | 1 856 896 | – | – | – | 1 | – | – |
| **AMUB–FRML** | 5 063 846 | 291 | 234 | 17 | 0.48 | 0.025 | N |
| **AMUB–ARML** | *11 003 356 | – | – | – | – | – | N |
| **FO–FRML** | *16 953 520 | – | – | – | – | – | Y |
| **MUB–FRML** | 19 227 538 | 9 | 0.00066 | 0.015 | 0.22 | 0.074 | N |
| **FO–ARML** | *27 016 438 | – | – | – | – | – | Y |
| **FOMUB–ARML** | *27 604 835 | – | – | – | – | – | Y |
| **FOMUB–FRML** | *34 353 230 | – | – | – | – | – | Y |
| **FMUB–FRML** | 38 348 155 | 27 | 0.0013 | 1 | 0.12 | 0.076 | Y |
| **FMUB–TRML** | 38 348 155 | 27 | 0.0013 | 1 | 0.12 | 0.076 | Y |
| **FMUB–FRLS** | 40 924 384 | 27 | 0.0022 | 0.56 | 0.11 | 0.067 | Y |
| **FMUB–PPI** | 41 797 578 | 27 | 0.0017 | 0.0028 | 0.11 | 0.068 | Y |
| **FMUB–CS** | 70 297 469 | 27 | 0.0027 | 0.63 | 0.074 | 0.091 | Y |
| **MUB–ARML** | 74 041 732 | 9 | 0.0011 | 0.7 | 0.1 | 0.14 | N |
| **PAULI–CS** | *203 019 460 | – | – | – | – | – | Y |
| **FMUB–ARML** | *227 858 692 | – | – | – | – | – | Y |

# 4 Random noisy preparation test

## 4.1 1 qubit

Table 37: Random noisy preparation test, 1 qubit, $F_B = 90\%$

| | $N_B$ | $M_B$ | $T_{P,B}$, sec | $T_{E,B}$, sec | $\eta_B$ | $O_B$ |
|---|---|---|---|---|---|---|
| **Lower bound** | 59 | – | – | – | 1 | – |
| **PAULI–CS** | *9 | – | – | – | – | – |
| **FMUB–CS** | *15 | – | – | – | – | – |
| **MUB–ARML** | *18 | – | – | – | – | – |
| **FMUB–ARML** | *18 | – | – | – | – | – |
| **MUB–FRML** | *19 | – | – | – | – | – |
| **FMUB–FRML** | *19 | – | – | – | – | – |
| **FMUB–TRML** | *19 | – | – | – | – | – |
| **FMUB–FRLS** | *19 | – | – | – | – | – |
| **FMUB–PPI** | *19 | – | – | – | – | – |
| **AMUB–FRML** | *25 | – | – | – | – | – |
| **AMUB–ARML** | *38 | – | – | – | – | – |

Table 38: Random noisy preparation test, 1 qubit, $F_B = 99\%$

| | $N_B$ | $M_B$ | $T_{P,B}$, sec | $T_{E,B}$, sec | $\eta_B$ | $O_B$ |
|---|---|---|---|---|---|---|
| **Lower bound** | 586 | – | – | – | 1 | – |
| **AMUB–FRML** | 1 051 | 13 | 0.042 | 0.012 | 0.72 | 0.029 |
| **AMUB–ARML** | 1 534 | 23 | 1.1 | 0.053 | 0.54 | 0.051 |
| **MUB–FRML** | 2 252 | 3 | 0.00026 | 0.0032 | 0.38 | 0.017 |
| **FMUB–FRML** | 2 252 | 3 | 0.00033 | 0.0029 | 0.38 | 0.017 |
| **FMUB–TRML** | 2 252 | 3 | 0.00033 | 0.0029 | 0.38 | 0.017 |
| **FMUB–FRLS** | 2 261 | 3 | 0.00031 | 0.37 | 0.37 | 0.017 |
| **FMUB–PPI** | 2 262 | 3 | 0.00041 | 0.00078 | 0.37 | 0.017 |
| **FMUB–CS** | 6 733 | 3 | 0.00042 | 0.53 | 0.13 | 0.0066 |
| **MUB–ARML** | 10 520 | 3 | 0.0005 | 0.01 | 0.12 | 0.1 |
| **FMUB–ARML** | 10 520 | 3 | 0.00049 | 0.0084 | 0.12 | 0.1 |
| **PAULI–CS** | 282 979 | 3 | 0.00038 | 0.69 | 0.0024 | 0.015 |

Table 39: Random noisy preparation test, 1 qubit, $F_B = 99.9\%$

| | $N_B$ | $M_B$ | $T_{P,B}$, sec | $T_{E,B}$, sec | $\eta_B$ | $O_B$ |
|---:|---:|---:|---:|---:|---:|---:|
| **Lower bound** | 5 861 | – | – | – | 1 | – |
| **AMUB–FRML** | 6 612 | 59 | 0.21 | 0.014 | 0.93 | 0.012 |
| **AMUB–ARML** | 7 088 | 60 | 1.3 | 0.12 | 0.88 | 0.017 |
| **MUB–FRML** | 27 014 | 3 | 0.00027 | 0.0031 | 0.3 | 0.037 |
| **FMUB–FRML** | 27 014 | 3 | 0.00033 | 0.0029 | 0.3 | 0.037 |
| **FMUB–TRML** | 27 014 | 3 | 0.00033 | 0.0029 | 0.3 | 0.037 |
| **FMUB–FRLS** | 27 014 | 3 | 0.00032 | 0.37 | 0.3 | 0.037 |
| **FMUB–PPI** | 27 014 | 3 | 0.00043 | 0.0008 | 0.3 | 0.037 |
| **MUB–ARML** | 50 048 | 3 | 0.00045 | 0.012 | 0.12 | 0.067 |
| **FMUB–ARML** | 50 048 | 3 | 0.00048 | 0.0098 | 0.12 | 0.067 |
| **FMUB–CS** | 84 784 | 3 | 0.00039 | 0.52 | 0.1 | 0.061 |
| **PAULI–CS** | *1 761 576 | – | – | – | – | – |

Table 40: Random noisy preparation test, 1 qubit, $F_B = 99.99\%$

| | $N_B$ | $M_B$ | $T_{P,B}$, sec | $T_{E,B}$, sec | $\eta_B$ | $O_B$ |
|---:|---:|---:|---:|---:|---:|---:|
| **Lower bound** | 58 610 | – | – | – | 1 | – |
| **AMUB–ARML** | 62 577 | 126 | 3.7 | 0.24 | 0.96 | 0.0034 |
| **AMUB–FRML** | 62 663 | 126 | 0.53 | 0.021 | 0.96 | 0.0032 |
| **MUB–FRML** | 264 308 | 3 | 0.00026 | 0.003 | 0.28 | 0.03 |
| **FMUB–FRML** | 264 308 | 3 | 0.00033 | 0.0029 | 0.28 | 0.03 |
| **FMUB–TRML** | 264 308 | 3 | 0.00033 | 0.0029 | 0.28 | 0.03 |
| **FMUB–FRLS** | 264 308 | 3 | 0.00032 | 0.36 | 0.28 | 0.03 |
| **FMUB–PPI** | 264 308 | 3 | 0.00043 | 0.00079 | 0.28 | 0.03 |
| **MUB–ARML** | 318 920 | 3 | 0.00047 | 0.024 | 0.16 | 0.039 |
| **FMUB–ARML** | 318 920 | 3 | 0.00046 | 0.02 | 0.16 | 0.039 |
| **FMUB–CS** | 704 194 | 3 | 0.0004 | 0.53 | 0.11 | 0.066 |
| **PAULI–CS** | *2 032 081 | – | – | – | – | – |

### 4.2 2 qubits

Table 41: Random noisy preparation test, 2 qubits, $F_B = 90\%$

| | $N_B$ | $M_B$ | $T_{P,B}$, sec | $T_{E,B}$, sec | $\eta_B$ | $O_B$ | FM |
|---|---|---|---|---|---|---|---|
| **Lower bound** | 312 | – | – | – | 1 | – | – |
| **AMUB–FRML** | *91 | – | – | – | – | – | N |
| **FMUB–FRML** | *128 | – | – | – | – | – | Y |
| **FMUB–TRML** | *128 | – | – | – | – | – | Y |
| **FMUB–FRLS** | *160 | – | – | – | – | – | Y |
| **MUB–FRML** | *173 | – | – | – | – | – | N |
| **FMUB–PPI** | *189 | – | – | – | – | – | Y |
| **FMUB–CS** | *196 | – | – | – | – | – | Y |
| **FOMUB–FRML** | *265 | – | – | – | – | – | Y |
| **FOMUB–ARML** | *361 | – | – | – | – | – | Y |
| **AMUB–ARML** | *377 | – | – | – | – | – | N |
| **FMUB–ARML** | *409 | – | – | – | – | – | Y |
| **MUB–ARML** | *634 | – | – | – | – | – | N |
| **FO–FRML** | 1 263 | 16 | 130 | 0.27 | 0.3 | 0.019 | Y |
| **FO–ARML** | 1 273 | 16 | 158 | 0.32 | 0.29 | 0.015 | Y |
| **PAULI–CS** | 3 868 | 15 | 0.0023 | 0.88 | 0.086 | 0 | Y |

Table 42: Random noisy preparation test, 2 qubits, $F_B = 99\%$

| | $N_B$ | $M_B$ | $T_{P,B}$, sec | $T_{E,B}$, sec | $\eta_B$ | $O_B$ | FM |
|---|---|---|---|---|---|---|---|
| **Lower bound** | 3 124 | – | – | – | 1 | – | – |
| **AMUB–FRML** | 15 089 | 83 | 2.5 | 0.27 | 0.27 | 0.021 | N |
| **FOMUB–FRML** | 24 257 | 103 | 8.9 | 1.5 | 0.17 | 0.022 | Y |
| **MUB–FRML** | 25 148 | 5 | 0.00066 | 0.036 | 0.16 | 0.014 | N |
| **FMUB–FRML** | 29 332 | 9 | 0.00053 | 0.14 | 0.13 | 0.012 | Y |
| **FMUB–TRML** | 29 332 | 9 | 0.00053 | 0.14 | 0.13 | 0.012 | Y |
| **FMUB–FRLS** | 36 378 | 9 | 0.0011 | 0.68 | 0.11 | 0.01 | Y |
| **FMUB–PPI** | 37 925 | 9 | 0.00062 | 0.00053 | 0.1 | 0.011 | Y |
| **AMUB–ARML** | 45 395 | 119 | 10 | 1.2 | 0.098 | 0.013 | N |
| **FO–FRML** | 47 114 | 115 | 164 | 0.65 | 0.11 | 0.013 | Y |
| **FMUB–CS** | 51 776 | 9 | 0.00087 | 0.5 | 0.07 | 0.016 | Y |
| **FO–ARML** | 70 197 | 127 | 218 | 2 | 0.058 | 0.024 | Y |
| **MUB–ARML** | 95 377 | 5 | 0.00072 | 0.16 | 0.051 | 0.081 | N |
| **FMUB–ARML** | 138 057 | 9 | 0.0012 | 0.21 | 0.036 | 0.1 | Y |
| **FOMUB–ARML** | 200 445 | 177 | 15 | 2.1 | 0.025 | 0.077 | Y |
| **PAULI–CS** | 5 021 781 | 15 | 0.0023 | 0.95 | 0.00079 | 0.072 | Y |

Table 43: Random noisy preparation test, 2 qubits, $F_B = 99.9\%$

| | $N_B$ | $M_B$ | $T_{P,B}$, sec | $T_{E,B}$, sec | $\eta_B$ | $O_B$ | FM |
|---|---|---|---|---|---|---|---|
| **Lower bound** | 31 245 | – | – | – | 1 | – | – |
| **AMUB–FRML** | 165 667 | 161 | 5.2 | 0.2 | 0.28 | 0.0083 | N |
| **FOMUB–FRML** | 629 755 | 218 | 36 | 2.1 | 0.095 | 0.036 | Y |
| **AMUB–ARML** | 965 051 | 219 | 46 | 5.1 | 0.1 | 0.11 | N |
| **MUB–FRML** | 1 016 042 | 5 | 0.00067 | 0.022 | 0.072 | 0.056 | N |
| **FMUB–FRML** | 1 251 861 | 9 | 0.00051 | 0.18 | 0.06 | 0.039 | Y |
| **FMUB–TRML** | 1 251 861 | 9 | 0.00051 | 0.18 | 0.06 | 0.039 | Y |
| **FMUB–FRLS** | 1 382 130 | 9 | 0.0011 | 0.66 | 0.05 | 0.038 | Y |
| **FMUB–PPI** | 1 400 187 | 9 | 0.00061 | 0.00057 | 0.049 | 0.038 | Y |
| **FMUB–CS** | 2 234 214 | 9 | 0.00091 | 0.49 | 0.027 | 0.014 | Y |
| **MUB–ARML** | 2 827 653 | 5 | 0.00071 | 0.31 | 0.03 | 0.062 | N |
| **FO–FRML** | 2 851 554 | 240 | 301 | 3.5 | 0.026 | 0.014 | Y |
| **FMUB–ARML** | 6 238 296 | 9 | 0.0012 | 0.47 | 0.017 | 0.13 | Y |
| **PAULI–CS** | *20 868 050 | – | – | – | – | – | Y |
| **FO–ARML** | *37 627 888 | – | – | – | – | – | Y |
| **FOMUB–ARML** | *88 879 631 | – | – | – | – | – | Y |

Table 44: Random noisy preparation test, 2 qubits, $F_B = 99.99\%$

| | $N_B$ | $M_B$ | $T_{P,B}$, sec | $T_{E,B}$, sec | $\eta_B$ | $O_B$ | FM |
|---|---|---|---|---|---|---|---|
| **Lower bound** | 312 447 | – | – | – | 1 | – | – |
| **AMUB–FRML** | 2 641 111 | 252 | 9.6 | 0.36 | 0.19 | 0.019 | N |
| **AMUB–ARML** | 4 471 818 | 269 | 124 | 13 | 0.14 | 0.047 | N |
| **FOMUB–FRML** | 5 763 044 | 296 | 54 | 1.9 | 0.093 | 0.038 | Y |
| **MUB–FRML** | 9 327 501 | 5 | 0.00061 | 0.0053 | 0.07 | 0.063 | N |
| **FMUB–FRML** | *10 010 497 | – | – | – | – | – | Y |
| **FMUB–TRML** | *10 010 497 | – | – | – | – | – | Y |
| **FMUB–PPI** | *10 765 217 | – | – | – | – | – | Y |
| **FMUB–FRLS** | *10 773 223 | – | – | – | – | – | Y |
| **FMUB–CS** | *12 042 970 | – | – | – | – | – | Y |
| **MUB–ARML** | *12 609 286 | – | – | – | – | – | N |
| **FMUB–ARML** | *17 458 991 | – | – | – | – | – | Y |
| **FO–FRML** | *18 236 562 | – | – | – | – | – | Y |
| **PAULI–CS** | *23 401 283 | – | – | – | – | – | Y |
| **FO–ARML** | *91 175 665 | – | – | – | – | – | Y |
| **FOMUB–ARML** | *322 473 430 | – | – | – | – | – | Y |

### 4.3 3 qubits

Table 45: Random noisy preparation test, 3 qubits, $F_B = 90\%$

| | $N_B$ | $M_B$ | $T_{P,B}$, sec | $T_{E,B}$, sec | $\eta_B$ | $O_B$ | FM |
|---|---|---|---|---|---|---|---|
| **Lower bound** | 1 857 | – | – | – | 1 | – | – |
| **MUB–FRML** | *177 | – | – | – | – | – | N |
| **AMUB–FRML** | *263 | – | – | – | – | – | N |
| **FMUB–FRML** | *423 | – | – | – | – | – | Y |
| **FMUB–TRML** | *423 | – | – | – | – | – | Y |
| **FOMUB–FRML** | *452 | – | – | – | – | – | Y |
| **FMUB–FRLS** | *975 | – | – | – | – | – | Y |
| **FO–FRML** | *990 | – | – | – | – | – | Y |
| **FMUB–CS** | *1 295 | – | – | – | – | – | Y |
| **FMUB–PPI** | *1 556 | – | – | – | – | – | Y |
| **AMUB–ARML** | *4 993 | – | – | – | – | – | N |
| **MUB–ARML** | *5 829 | – | – | – | – | – | N |
| **FO–ARML** | *7 414 | – | – | – | – | – | Y |
| **FMUB–ARML** | *9 197 | – | – | – | – | – | Y |
| **FOMUB–ARML** | *9 564 | – | – | – | – | – | Y |
| **PAULI–CS** | 400 226 | 63 | 0.0063 | 0.89 | 0.006 | 0 | Y |

Table 46: Random noisy preparation test, 3 qubits, $F_B = 99\%$

| | $N_B$ | $M_B$ | $T_{P,B}$, sec | $T_{E,B}$, sec | $\eta_B$ | $O_B$ | FM |
|---|---|---|---|---|---|---|---|
| **Lower bound** | 18 569 | – | – | – | 1 | – | – |
| **AMUB–FRML** | 74 506 | 143 | 256 | 68 | 0.28 | 0.019 | N |
| **FOMUB–FRML** | 164 533 | 212 | 626 | 488 | 0.12 | 0.018 | Y |
| **MUB–FRML** | 167 081 | 9 | 0.0012 | 0.8 | 0.12 | 0.016 | N |
| **FO–FRML** | 196 801 | 159 | 2 772 | 55 | 0.11 | 0.015 | Y |
| **FMUB–FRML** | 215 852 | 27 | 0.0014 | 1.1 | 0.095 | 0.018 | Y |
| **FMUB–TRML** | 215 852 | 27 | 0.0014 | 1.1 | 0.095 | 0.018 | Y |
| **FMUB–FRLS** | 317 195 | 27 | 0.0026 | 0.63 | 0.065 | 0.019 | Y |
| **FMUB–CS** | 351 892 | 27 | 0.0037 | 0.87 | 0.06 | 0.018 | Y |
| **FMUB–PPI** | 376 265 | 27 | 0.0017 | 0.0025 | 0.056 | 0.018 | Y |
| **AMUB–ARML** | 611 077 | 217 | 3 229 | 786 | 0.041 | 0.018 | N |
| **MUB–ARML** | 644 405 | 9 | 0.00099 | 1.5 | 0.036 | 0.045 | N |
| **FMUB–ARML** | 908 286 | 27 | 0.0023 | 2 | 0.025 | 0.022 | Y |
| **FO–ARML** | 1 136 683 | 212 | 1 | 454 | 0.021 | 0.0058 | Y |
| **FOMUB–ARML** | 1 969 515 | 321 | 2 936 | 1 638 | 0.013 | 0.0046 | Y |
| **PAULI–CS** | 72 751 747 | 63 | 0.0062 | 0.93 | 0.00032 | 0.014 | Y |

Table 47: Random noisy preparation test, 3 qubits, $F_B = 99.9\%$

| | $N_B$ | $M_B$ | $T_{P,B}$, sec | $T_{E,B}$, sec | $\eta_B$ | $O_B$ | FM |
|---|---|---|---|---|---|---|---|
| **Lower bound** | 185 690 | – | – | – | 1 | – | – |
| **AMUB–FRML** | 1 317 030 | 244 | 1 067 | 66 | 0.19 | 0.009 | N |
| **MUB–FRML** | 12 349 241 | 9 | 0.0012 | 0.75 | 0.027 | 0.0047 | N |
| **FO–FRML** | *13 688 307 | – | – | – | – | – | Y |
| **FOMUB–FRML** | *14 320 719 | – | – | – | – | – | Y |
| **AMUB–ARML** | *15 420 416 | – | – | – | – | – | N |
| **FMUB–FRML** | 18 382 472 | 27 | 0.0013 | 2 | 0.019 | 0.016 | Y |
| **FMUB–TRML** | 18 382 472 | 27 | 0.0013 | 2 | 0.019 | 0.016 | Y |
| **FMUB–FRLS** | 22 250 404 | 27 | 0.0025 | 0.62 | 0.014 | 0.01 | Y |
| **FMUB–PPI** | 23 467 175 | 27 | 0.0016 | 0.0025 | 0.014 | 0.0093 | Y |
| **FMUB–CS** | 29 173 307 | 27 | 0.0039 | 0.91 | 0.011 | 0.0083 | Y |
| **MUB–ARML** | 39 838 333 | 9 | 0.00097 | 9 | 0.013 | 0.082 | N |
| **FOMUB–ARML** | *84 818 569 | – | – | – | – | – | Y |
| **FMUB–ARML** | *104 503 809 | – | – | – | – | – | Y |
| **PAULI–CS** | *324 383 666 | – | – | – | – | – | Y |
| **FO–ARML** | *386 192 651 | – | – | – | – | – | Y |

Table 48: Random noisy preparation test, 3 qubits, $F_B = 99.99\%$

| | $N_B$ | $M_B$ | $T_{P,B}$, sec | $T_{E,B}$, sec | $\eta_B$ | $O_B$ | FM |
|---|---|---|---|---|---|---|---|
| **Lower bound** | 1 856 896 | – | – | – | 1 | – | – |
| **AMUB–FRML** | *11 965 326 | – | – | – | – | – | N |
| **AMUB–ARML** | *22 314 118 | – | – | – | – | – | N |
| **FO–FRML** | *26 032 648 | – | – | – | – | – | Y |
| **FOMUB–FRML** | *29 807 799 | – | – | – | – | – | Y |
| **FOMUB–ARML** | *121 605 576 | – | – | – | – | – | Y |
| **MUB–FRML** | *126 680 555 | – | – | – | – | – | N |
| **FMUB–FRML** | *145 112 112 | – | – | – | – | – | Y |
| **FMUB–TRML** | *145 112 112 | – | – | – | – | – | Y |
| **FMUB–PPI** | *148 667 382 | – | – | – | – | – | Y |
| **FMUB–FRLS** | *152 226 642 | – | – | – | – | – | Y |
| **FMUB–CS** | *160 348 622 | – | – | – | – | – | Y |
| **MUB–ARML** | *163 088 332 | – | – | – | – | – | N |
| **FMUB–ARML** | *208 389 099 | – | – | – | – | – | Y |
| **PAULI–CS** | *372 190 386 | – | – | – | – | – | Y |
| **FO–ARML** | *689 799 681 | – | – | – | – | – | Y |
